# Supplementary material for: Neural Networks Regularization Through Representation Learning
Source: arXiv:1807.05292 source file (2018-07-13)
Supplement: Supplementary file 1 [file appendix1.tex]

% ******************************* Thesis Appendix A ****************************
% Appendix A: related to the chapter "machine learning".
\chapter{Machine Learning}  %Title of the First Chapter
\label{chap:chapterapp1}

\ifpdf
    \graphicspath{{Appendix1/Figs/Raster/}{Appendix1/Figs/PDF/}{Appendix1/Figs/}}
\else
    \graphicspath{{Appendix1/Figs/Vector/}{Appendix1/Figs/}}
\fi

\makeatletter
\def\input@path{{Appendix1/}}
\makeatother

We discuss in this appendix further details on machine learning aspects which we have presented in Sec.\ref{sec:machinel0}. We illustrate the use of machine learning throughout its applications in real life and give some problems that can be solved by using it (Sec.\ref{sec:applicationsandproblemsapp1}). Next, we provide some basic definitions (Sec.\ref{sec:definitionsandterminologyapp1}) and different learning scenarios in machine learning (Sec.\ref{sec:learningscenariosapp1}). In Sec.\ref{sec:learningandoptimapp1}, we tackle learning problems from optimization point of view where we describe gradient descent based methods which we used in our contributions in this thesis. At the end of this appendix (Sec.\ref{sec:learningandgeneralizationapp1}), we discuss further related subjects to the generalization theory (Sec.\ref{sub:generalizationtheoryapp1}) including VC-dimension (Sec.\ref{sub:generalizationtheoryapp1}), bias-variance tradeoff (Sec.\ref{sub:biasvarianceapp1}), and regularization (Sec.\ref{sub:regularizationappapp1}).

\section{Applications}
\label{sec:applicationsandproblemsapp1}
Machine learning algorithms have been successfully deployed in a variety of applications, including
\begin{itemize*}
    \item Text or document classification, e.g., spam detection;
    \item Natural language processing, e.g., part-of-speech tagging, statistical parsing, name-entity recognition;
    \item Speech recognition, speech synthesis, speaker verification;
    \item Computational biology applications, e.g., protein function or structural prediction;
    \item Computer vision tasks, e.g., image recognition, face detection;
    \item Fraud detection (credit card, telephone), and network intrusion;
    \item Games, e.g., chess, backgammon, go;
    \item Unassisted vehicle control (robots, navigation);
    \item Medical diagnosis;
    \item Recommendation systems, search engines, information extraction systems.
\end{itemize*}

This list is by no means comprehensive, and learning algorithms are applied to new applications every day. Moreover, such applications correspond to a wide variety of learning problems. Some major classes of learning problems are:
\begin{itemize}
    \item \emph{Classification}: Assign a category to each item. For example, document classification may assign items with categories such as \emph{politics}, \emph{business}, \emph{sports}, or \emph{weather}.
    \item \emph{Regression}: Predict a real value for each item. Examples of regression include prediction of stock values or variations of economic variables. In this problem, the penalty for an incorrect prediction depends on the magnitude of difference between the true and predicted values.
    \item \emph{Ranking}: Order items according to some criterion. Web search, e.g., returning web pages relevant to a search query, is the canonical ranking example.
    \item \emph{Clustering}: Partition items into homogeneous regions. Clustering is often performed to analyze very large data sets. For example, in the context of social network analysis, clustering algorithms attempt to identify \quotes{communities} within large groups of people.
    \item \emph{Dimensionality reduction or manifold learning}: Transform an initial representation of items into a lower-dimensional representation of the items while preserving some properties of the initial representation. A common example involves preprocessing digital images in computer vision tasks.
\end{itemize}

In the next section, we provide basic definitions and terminology of machine learning.

\section{Definitions and Terminology}
\label{sec:definitionsandterminologyapp1}
Let us use the canonical problem of spam detection as a running example to illustrate some basic definitions and to describe the use and evaluation of machine learning algorithms in practice \cite{Mohri2012bookML}. Spam detection is the problem of learning to automatically classify email messages as either \texttt{SPAM} or \texttt{not-SPAM}.

\begin{itemize}
    \item \emph{Examples}: Items or instances of data used for learning or evaluation. In our spam problem, these examples correspond to the collection of email messages we will use for learning and testing.
    \item \emph{Features}: The set of attributes, often represented as a vector, associated to an example. In the case of email messages, some relevant features may include the length of the message, the name of the sender, various characteristics of the header, the presence of certain keywords in the body of the message, and so on.
    \item \emph{Labels}: Values or categories assigned to examples. In classification problems, examples are assigned specific categories, for instance, the \texttt{SPAM} and \texttt{not-SPAM} categories in our binary classification problem. In regression, items are assigned real-valued labels.
    \item \emph{Training samples}: Examples used to train a learning algorithm. In our spam problem, the training samples consist of a set of email examples along with their associated labels.
    \item \emph{Validation samples}: Examples used to tune the parameters of a learning algorithm when working with labeled data. Learning algorithms typically have one or more free parameters, and the validation samples are used to select appropriate values for these model parameters.
    \item \emph{Test samples}: Examples used to evaluate the performance of a learning algorithm. The test samples are separate from the training and validation data and is not made available in the learning stage. In the spam problem, the test samples consist of a collection of email examples for which the learning algorithm must predict labels based on features. These predictions are then compared with the labels of the test samples to measure the performance of the algorithm.
    \item \emph{Loss function}: A function that measures the difference, or loss, between a predicted label and a true label. Denoting the set of all labels as $\Y$ and the set of possible predictions as $\Y^{\prime}$, a loss function ${\ell: \Y^{\prime} \times \Y \to \R_{+}}$. In most cases, $\Y^{\prime} = \Y$ and the loss function is bounded, but these conditions do not always hold. Common examples of loss functions include the zero-one (or misclassification) loss defined over $\{-1, +1\} \times \{-1, +1\}$ by $\ell(y^{\prime}, y) = \ind_{y^{\prime} \neq y}$ and the squared loss defined over $I \times I$ by ${\ell(y^{\prime}, y) = (y^{\prime} - y)^2}$, where $I \subseteq \R$ is typically a bounded interval.
    \item \emph{Hypothesis set}: A set of functions mapping features (feature vectors) to the set of label $\Y$. In our example, these may be a set of functions mapping email features to $\Y = \{\text{\texttt{SPAM }}, \text{\texttt{not-SPAM}}\}$. More generally, hypotheses may be functions mapping features to a different set $\Y^{\prime}$. They could be linear functions mapping email feature vector to real numbers interpreted as scores ($\Y = \R$), with higher score values more indicative of $\texttt{SPAM}$ than lower ones.
\end{itemize}

We now define the learning stages of our spam problem. We start with a given collection of labeled examples. We first randomly partition the data into  training samples, validation samples, and  test samples. The size of each of these samples depends on a number of different considerations. For example, the amount of data reserved for validation depends on the number of free parameters of the algorithm. Also, when labeled samples are relatively small, the amount of training data is often chosen to be larger than that of test data since the learning performance directly depends on the training samples.

Next, we associate relevant features to the examples. This is a critical step in the design of machine learning solutions. Useful features can effectively guide the learning algorithm, while poor or uninformative ones can be misleading. Although it is critical, to a large extent, the choice of the features is left to the user. This choice reflects the user's prior knowledge about the learning task which in practice can have a dramatic effect on the performance results.

Now, we use the features selected to train our learning algorithm by fixing different values of its free parameters. For each value of these parameters, the algorithm selects a different hypothesis out of the hypothesis set. We choose among them the hypothesis resulting in the best performance on the validation samples. Finally, using that hypothesis, we predict the labels of the examples in the test samples. The performance of the algorithm is evaluated by using the loss function associated to the task, e.g., the zero-one loss in our spam detection task, to compare the predicted and true value.

Thus, the performance of an algorithm is of course evaluated based on its test error and not its error on the training samples. A learning algorithm may be consistent, that is it may commit no error on the examples of the training data, and yet have a poor performance on the test data. This occurs for consistent learners defined by very complex decision surfaces, as illustrated in Fig.\ref{fig:fig0-0}, which tend to memorize a relatively small training samples instead of seeking to generalize well. This highlights the key distinction between memorization and generalization, which is the fundamental property sought for an accurate learning algorithm.

\begin{figure}[!htbp]
  % \centering
  % \includegraphics[scale=0.3]{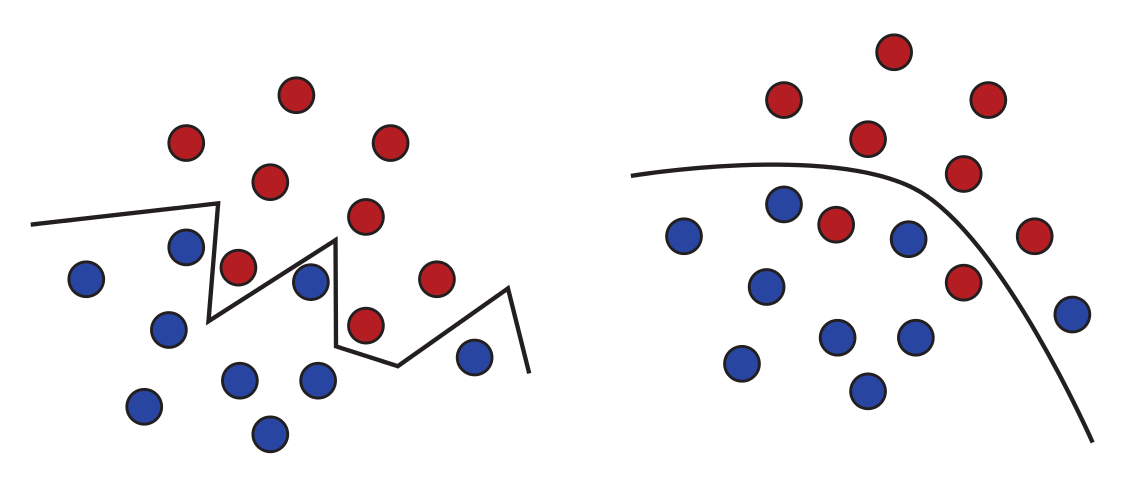}
  \begin{center}
		\input{consistentlearner}
	\end{center}
  \caption[\bel{Complexity vs. generalization.}]{The zig-zag line on the left panel is consistent over the blue and red training samples, but it is a complex separation surface that is not likely to generalize well to unseen data. In contrast, the decision surface on the right panel is simpler and might generalize better in spite of its misclassification of few points of the training samples. (Reference:  \cite{Mohri2012bookML})}
  \label{fig:fig0-0}
\end{figure}

In the following, we describe some common learning scenarios.

\section{Learning Scenarios}
\label{sec:learningscenariosapp1}
We briefly describe common machine learning scenarios \cite{Mohri2012bookML}. These scenarios differ in the type of training data available to the learner, the order and method by which training data is received and the test data used to evaluate the learning algorithm.

\begin{itemize}
    \item \emph{Supervised learning}: The learner receives a set of labeled examples as training data and makes predictions for all unseen points. This is the most common scenario associated with classification, regression, and ranking problems.
    \item \emph{Unsupervised learning}: The learner exclusively receives unlabeled training data, and makes prediction for all unseen points. Since in general no labeled example is available in that setting, it can be difficult to quantitatively evaluate the performance of a learner. Clustering and dimensionality reduction are example of unsupervised learning problems.
    \item \emph{Semi-supervised learning}: The learner receives some training samples which consist of both labeled and unlabeled data, and makes predictions for all unseen points. Semi-supervised learning is common in setting where unlabeled data is easily accessible but labels are expensive to obtain. Various types of problems arising in applications, including classification, regression, or ranking tasks, can be framed as instances of semi-supervised learning. The hope is that the distribution of unlabeled data accessible to the learner can help to achieve a better performance than in the supervised setting.
    \item \emph{Transductive inference}: As in the semi-supervised scenario, the learner receives labeled training samples along with a set of unlabeled test points. However, the objective of transductive inference is to predict labels only for these particular test points. Transductive inference appears to be an easier task and matches the scenario encountered in a variety of modern applications. However, the assumptions under which a better performance can be achieved in this setting are research questions that have not been fully solved.
    \item \emph{Online learning}: In contrast with the previous scenarios, the online scenario involves multiple rounds and training and testing phases are intermixed. At each round, the learner receives an unlabeled training point, makes a prediction, receives the true label, and incurs a loss. The objective in the online setting is to minimize the cumulative loss over all rounds. Unlike the previous settings just discussed, no distributional assumption is made in online learning.
    \item \emph{Reinforcement learning}: The training and the testing phases are also intermixed in reinforcement learning. To collect information, the learner actively interacts with the environment and in some cases affects the environment, and receives an immediate reward for each action. The object of the learner is to maximize his reward over a course of actions and iterations with the environment. However, no long-term reward feedback is provided by the environment, and the learner is faced with the exploration versus exploitation dilemma, since he must choose between exploring unknown actions to gain more information versus exploiting the information already collected.
    \item \emph{Active learning}: The learner adaptively or interactively collects training examples, typically by querying an orcale to request labels for new points. The goal in active learning is to achieve a performance comparable to the standard supervised learning scenario, but with fewer labeled examples. Active learning is often used in applications where labels are expensive to obtain, for example computational biology applications.
\end{itemize}
In practice, many other intermediate and somewhat more complex learning scenarios may be encountered.

In the following section, we cast the learning problem as an optimization problem. We present maximum likelihood estimation and gradient based optimization methods.

\section{Learning and Optimization}
\label{sec:learningandoptimapp1}

For the sake of simplicity, let us consider the supervised learning case. Let $\X$ be an input space, $\Y$ be the output space. $p_{data}$ is the data generating distribution over $\X \times \Y$ that describes the data we observe. $f \in \mathbb{F}$ is a function: $f: \X \to \Y$, parameterized with the set of parameters $\bm{\theta}$ drawn from the parameters space $\Theta$. $\ell(., .)$ is the per-example loss function.

In order to choose the best approximation function $f$, one need to minimize the expected value of the loss $\ell$ defined as \cite{Goodfellowbook2016}
\begin{equation}
\label{eq:eqapp1-0}
J^*(\bm{\theta}) = \mathop{\mathbb{E}}_{(\x, \y) \sim p_{data}} [\ell(f(\xvec;\bm{\theta}), \yvec)] \; .
\end{equation}
\noindent The quantity Eq.\ref{eq:eqapp1-0} is know as the risk functional. It is a simple way to convert a machine learning problem to an optimization problem.

In practice, the true distribution $p_{\text{data}}$ is unknown. However, we can replace it with an empirical distribution $\hat{p}_{\text{data}}$ defined by a set of $m$ training samples: independent and identically distributed (i.i.d). Now, the empirical risk $J$ is minimized instead \cite{Goodfellowbook2016}
\begin{equation}
\label{eq:eqapp1-1}
J(\bm{\theta}) = \mathop{\mathbb{E}}_{(\x,\y) \sim \hat{p}_{\text{data}}}[\ell(f(\xvec; \bm{\theta}), \yvec)] = \frac{1}{m} \sum^m_{i=1} \ell(f(\xvec^{(i)}; \bm{\theta}), \yvec^{(i)}) \; ,
\end{equation}

Therefore, the learning process can be simply described as an optimization problem to find the optimum parameters $\bm{\theta}$
\begin{equation}
\label{eq:eqapp1-2}
\begin{aligned}
& \underset{\bm{\theta} \in \Theta}{\text{minimize}}
& & J(\bm{\theta})  \quad \text{(Eq.\ref{eq:eqapp1-1})} \; .
\end{aligned}
\end{equation}
All along our contributions in this thesis, we will be using maximum likelihood method to find the optimum parameters which we will describe in the next section.

\subsection{Maximum Likelihood Estimation (MLE)}
\label{sub:mleappa1}
Before tackling the maximum likelihood procedure, an important aspect about the data samples should be highlighted.

In order to evaluate a learned model, one needs a different set of samples: the test set $\mathbb{D}_{\text{text}}$ which is a set of $m$  samples not seen during the learning process. Measuring the model's performance over $\mathbb{D}_{\text{text}}$  gives us an evaluation of the capability of the model $f$ to generalize to new samples. Generalization is a vital aspect of machine learning and one of the concept that makes it different from pure optimization. More about generalization will be discussed in Sec.\ref{sub:generalizationtheoryapp1}.

In order to be able to generalize from training data to test data, one needs to assume that there is a common structure in the data. One of the most important assumption is that the data is independently and identically distributed (i.i.d.). This means that each sample is generated independently from other samples and all the samples are generated from the same distribution $p_{\text{data}}$. Given the set of $m$ samples under the form of a $m \times n$ matrix $\bm{X}$, this i.i.d. idea can be expressed as \cite{Goodfellowbook2016}

\begin{equation}
\label{eq:eqapp1-3}
p_{\text{data}}(\mathbf{X}, \y) = \prod_i p_{\text{data}}(\bm{X}_{i,:}, \yvec^{(i)}) \; , 
\end{equation}
\noindent wwhere $\bm{y}^{(i)}$ is the label of the $i$-th  input sample. Eq.\ref{eq:eq0-3} is known as the likelihood function.

\bigskip
In statistics, maximum likelihood estimation is a well known method for estimating the parameters of a model given observations generated from an unknown distribution $p_{\text{data}}$. The approach defines a probabilistic model parametrized by a set of parameters $\bm{\theta}$. Then, a probability distribution can be defined over the observations $\mathbf{x}$: $p_{\text{model}}(\mathbf{x}; \bm{\theta})$. Using a statistical estimator, one can find the good value of $\bm{\theta}$ drawn from all the possible values $\Theta$.

The MLE defines the best estimated parameter, noted $\bm{\hat{\theta}}$, as \cite{Goodfellowbook2016}
\begin{equation}
    \label{eq:eqapp1-4}
    \bm{\hat{\theta}} = \argmax_{\bm{\theta} \in \Theta} \prod_i p_{\text{model}}(\bm{X}_{i,:};\bm{\theta}) \; .
\end{equation}

The MLE procedure picks the parameters that maximize the probability that the observed data are generated by the model.

One of the properties of MLE is that the provided solution is invariant to a strictly monotone increasing function of the likelihood function (Eq.\ref{eq:eqapp1-3}) such as the logarithm function. In practice, we usually use the log-likelihood \cite{Goodfellowbook2016}
\begin{equation}
    \label{eq:eqapp1-5}
    \bm{\hat{\theta}} = \argmax_{\bm{\theta} \in \Theta} \sum_i \log p_{\text{model}}(\bm{X}_{i,:};\bm{\theta}) \; .
\end{equation}
\noindent Turning the product to a sum over the samples is more convenient in mathematical analysis. Moreover, computing the product of small values $[0, 1]$ over a computer can lead to underflow. Therefore, it is common to use in practice the log-likelihood instead of the likelihood \cite{Goodfellowbook2016}.

Assuming that the true distribution ${p_{\text{data}} \in \{p_{\text{model}}(\mathbf{x}; \bm{\theta}), \bm{\theta} \in \Theta\}}$. The MLE picks the one model which maximizes the likelihood. This recovers a model distribution $p_{\text{model}}$ which matches the true distribution $p_{\text{data}}$. However, it is not guaranteed  to recover the true parameters \cite{Goodfellowbook2016}. Under some conditions, the MLE provides asymptotically (i.e., when the number of training samples is infinite), to the true parameters. For one, there may be more than one parameter that maximizes the likelihood function. Therefore, the true parameter can not be determined \citep{NEWEY19942111}.

A well known issue of MLE is the overfitting which is the case when the model is unable to generalize for unseen samples. The maximum likelihood estimator performs well in the case of infinite data. In the case of finite data, which is the practical case, it is not always the best approach \cite{Goodfellowbook2016}. When few training samples are available, the maximum likelihood performs poorly. This can be alleviated by combining the MLE with a Bayesian inference such as the Maximum A Posteriori estimation (MAP). One can see the MAP as a regularized MLE which allows to set a prior about the parameters. Regularized MLE has roughly the same computation cost as the unregularized one but it performs better \cite{Goodfellowbook2016}. Typically, the solution of the regularized MLE consists in finding a solution that maximize the likelihood function of the data given the parameter $\bm{\theta}$ and at the same time the likelihood of the parameter $\bm{\theta}$ under some prior. We discuss more details about regularization in Sec.\ref{sec:learningandgeneralizationapp1}. Along this thesis, we use the regularized MLE in most cases.

In supervised learning, the aim is to learn a parameterized function $f(\xvec;\bm{\theta})$ that maps the input space $\X$ to the output space $\Y$ to perform different tasks such as the classification or the regression task. One usually seeks to model the joint distribution $p(\x, \y; \bm{\theta})$ which can be simplified under the i.i.d. condition to the conditional distribution $p(\y|\x; \bm{\theta})$. Using the MLE, one can fit a model to $p(\y|\x; \bm{\theta})$ using the training data and by setting $f(\xvec) = \argmax\limits_{\yvec} p(\yvec|\xvec)$.

The classification task can be solved using the log-likelihood estimator as follows \cite{Goodfellowbook2016}
\begin{equation}
    \label{eq:eqapp1-6}
    \bm{\hat{\theta}} = \argmax_{\bm{\theta}} \sum_i \log p_{\text{model}}(\xvec^{(i)}, \yvec^{(i)}; \bm{\theta}) \; .
\end{equation}

In the case of regression, it can be shown \citep{Bishop2006}, under some assumptions, that the solution to MLE can be written as the sum-of-squares error function:

\begin{equation}
    \label{eq:eqapp1-7}
    \bm{\hat{\theta}} = \argmin_{\bm{\theta}} \sum_i \norm{\yvec^{(i)} - f(\xvec^{(i)}; \bm{\theta})}^2 \; .
\end{equation}

\subsection{Optimization}
\label{sub:optimizationapp1}

We recall from Sec.\ref{sec:learningandoptimapp1}, that a learning problem can be cast as an optimization problem. When using the maximum likelihood estimation, an objective function to be optimized can be defined as follows \cite{Goodfellowbook2016}
\begin{equation}
\label{eq:eqapp1-8}
\begin{aligned}
& \underset{\bm{\theta} \in \Theta}{\text{maximize}}
& & J(\bm{\theta}) = \sum_i \log p_{\text{model}}(\bm{X}_{i,:}; \bm{\theta}) \; .
\end{aligned}
\end{equation}

Assuming that the function $f(\xvec; \bm{\theta}) = p_{\text{model}}(\xvec;\bm{\theta})$ implemented by the model and the cost function are both differentiable. Solving such an optimization problem is usually done by exploiting the gradient of the objective function. In some cases, the solution can be obtained analytically by solving: $\nabla_{\bm{\theta}}J(\bm{\theta}) = 0$ for $\bm{\theta}$. However, in most cases, the analytic solution can be difficult to obtain or even impossible \cite{Goodfellowbook2016}. Usually, one can use iterative optimization methods which approximate the solution iteratively starting from an initial guess. We will be using this approach all along this thesis.

Gradient ascent is one of the simplest iterative methods used to solve such an optimization problem. It is based on the observation that $\nabla_{\bm{\theta}}J(\bm{\theta})$ indicates the direction in which the cost function $J(\bm{\theta})$ increases the most rapidly in a local neighborhood round $\bm{\theta}$. In order to find the maximum of the optimization (Eq.\ref{eq:eqapp1-8}), gradient ascent suggests to take a small step toward the direction of the gradient \citep{Bishop2006}. At the iteration $t$ of the gradient ascent algorithm, the parameter update can be computed using the following rule \cite{Goodfellowbook2016}

\begin{equation}
    \label{eq:eqapp1-8-1}
    \bm{\theta}^{(t)} \coloneqq \bm{\theta}^{(t-1)} + \eta(t) \nabla_{\bm{\theta}}J(\bm{\theta}) \; ,
\end{equation}
\noindent where $\eta(t)$ is a positive scalar which controls the size of the step, hence, the speed of learning. It is a tunable-dependent parameter that has a considerable impact on the optimization. It is commonly known as the learning rate. Alg.\ref{alg:algapp1-0} shows a sketch of the gradient ascent algorithm.

\begin{algorithm}[!htbp]
    \begin{algorithmic}[1]
      \State $t=0$. $\bm{\theta}^{0}$ is an initial guess. 
      \For{iterations}
       \State $t \coloneqq t + 1$
       \State $\bm{\theta}^{(t)} \coloneqq \bm{\theta}^{(t-1)} + \eta(t) \nabla_{\bm{\theta}}J(\bm{\theta})$
      \EndFor
    \end{algorithmic}
    \caption{A sketch of the gradient ascent algorithm.}
    \label{alg:algapp1-0}
\end{algorithm}

The strategy used to compute the gradient in Eq.\ref{eq:eqapp1-8-1} involves the processing of the whole training dataset at once. This is referred to as batch training. This can be inefficient when there is redundant samples in the training set. More importantly, it can be computationally costly when dealing with large training datasets. It may be worthwhile to use sequential training, also known as online training, where the data samples are considered one at a time. The model's parameters are updated after each sample presentation. This processing strategy is more appropriate in the case where the data samples arrive in a continuous stream. This type of training algorithm is referred to as stochastic gradient ascent. Online training can take too long especially for large training datasets. Moreover, the estimated gradient at each sample can be very noisy. A compromise training strategy between batch training and online training is referred to as mini-batch training, where one can take only few random samples from training set to estimate the direction of the gradient. The update rule in Eq.\ref{eq:eqapp1-8-1} is re-written as follows \cite{Goodfellowbook2016}

\begin{equation}
    \label{eq:eqapp1-9}
    \bm{\theta}^{(t)} \coloneqq \bm{\theta}^{(t-1)} + \eta(t) \nabla_{\bm{\theta}} \sum_{i \in \mathbb{B}} \log p_{\text{model}}(\bm{X}_{i,:}; \bm{\theta}) \; ,
\end{equation}
\noindent where $\mathbb{B}$ is a random subset of $\{1, \dots, m\}$. The size of the mini-batch is a hyper-parameter of the optimization problem that the user needs to set. Nowadays, most applications use the mini-batch strategy due to its advantages. For one, it is fast to compute and it allows to reduce redundant computations. Although, the estimated gradient is still noisy but it may be helpful to \quotes{push} the model from poor local maxima hopefully to regions with global maxima.

Gradient ascent can be enhanced using a technique called momentum \citep{Nesterov1983wy} which uses the gradient information to update the model's parameters. Instead of following the steepest direction at each step when using gradient ascent, momentum follows a direction by accumulating speed in directions that consistently maximizes the cost function. Formally, a momentum method maintains a velocity vector $\bm{v}^{(t)}$ that is influenced by the gradient at each step as follows \cite{Goodfellowbook2016}

\begin{align}
\bm{v}^{(t)} & \coloneqq \mu(t) \bm{v}^{t-1} + \eta(t) \nabla_{\bm{\theta}}\sum_{i \in \mathbb{B}} \log p_{\text{model}}(\bm{X}_{i,:}; \bm{\theta}) \label{eq:eqapp1-10-0} \; , \\
 \bm{\theta}^{(t)} & \coloneqq \bm{\theta}^{(t-1)} + \bm{v}^{(t)} \; , \label{eq:eqapp1-10}
\end{align}
\noindent where $\mu(t)$ is a decay coefficient $[0, 1]$. It is a tunable-parameter to control the rate at which the old gradient is considered. Its physical interpretation is the \quotes{friction} of the surface of the objective function. \citep{sutskever1} showed that momentum method can perform as well as second order methods like Hessian-free optimization \citep{Martens10, Nocedal2006NO}.

\bigskip

Up to now, we have described the optimization problem in terms of ascending the log-likelihood function seeking a maximum. However, in practice, it is common to search a minimum of an objective function. Stochastic Gradient Descent (SGD) is one of the methods used for this purpose. In this case, the learning rule is presented as a descending cost function. Therefore, instead of using the log-likelihood to maximize, the negative log-likelihood function is used instead to minimize.

In practice, two main ways can be used to influence the solution of the optimization problem using gradient method. The first one is the learning rate function $\eta(t)$ (and $\mu(t)$ when using momentum method) which determines the speed of convergence. The value of the learning rate must be picked carefully and it is better to adapt it through the learning procedure. Smaller values can lead to slow learning while large values can lead to divergence of the learning. The second most important way to control the solution of the optimization problem is the convergence criterion which indicates that the learning must stop. One can decide to halt the learning process when $J(\bm{\theta})$, evaluated over a held-out validation set, does not decrease (when using SGD), after some training time.

Another intuitive way to halt the training is when the gradient on the training set is close to zero indicating a local minima. However, it is an impractical method because it usually results in overfitting \cite{Goodfellowbook2016}, a situation that occurs when the model memorizes the patterns in the training set. By falling in this situation, we prevent the model from generalization over unseen samples. This is a crucial goal in machine learning where the aim is to build a model capable to perform well over unseen data. We dedicate the next section to discuss, from a theoretical perspective, the issue of overfitting and how to deal with it to train models that generalize better.

\section{Learning and Generalization}
\label{sec:learningandgeneralizationapp1}

So far, we have presented machine learning as an optimization problem. This is partially true. In fact, the core of machine learning is the ability to learn which is the capability to perform well over new unseen samples. This is referred to as generalization which is a central problem in machine learning. In this section, we present the generalization theory, the bias-variance tradeoff, and describe the regularization concept which is one of the most successful strategy to deal with the overfitting problem.

\subsection{Generalization Theory}
\label{sub:generalizationtheoryapp1}

In Sec.\ref{sec:learningandoptimapp1}, we defined the learning concept as the expected value of the error of the model $f(\bm{x};\bm{\theta})$ over a training set $\mathbb{D}_{\text{train}} \sim \hat{p}(\x, \y)$ (Eq.\ref{eq:eqapp1-1}). This definition does not show the true meaning of learning. So fare, we defined an optimization problem.

The central challenge in machine learning is to give the learned machine the ability to perform well on new samples. In the field of statistical learning, this ability is named generalization which holds the real meaning of learning.

In order to understand the generalization concept we need to take a look to our data.

The empirical risk in Eq.\ref{eq:eqapp1-0} is defined over all the possible samples $(\x, \y)$ generated by an unknown distribution $p_{\text{data}}$ named the data generating process. If $p_{\text{data}}$ is known, the learning problem is solved.  However, $p_{\text{data}}$ is unknown and it is approximated by $\hat{p}_{\text{data}}$ which is defined by a finite set of samples $\mathbb{D}$. In this case, we consider a very important assumption about the available samples which will make the learning possible. We consider that all the samples are drawn independently from each other and they all have been drawn from the same distribution $\hat{p}_{\text{data}}$.

From the set $\mathbb{D}$, we draw two separate sets.The train set $\mathbb{D}_{\text{train}}$ and the test $\mathbb{D}_{\text{test}}$ with no overlap between them. Using the empirical risk, the model error over both sets is defined as 
\begin{equation}
    \label{eq:eqapp1-13}
    E_{\mathbb{D}_{\text{train}}} = \E_{(\xvec,\yvec) \in \mathbb{D}_{\text{train}}}[\ell(f(\xvec; \bm{\theta}), \yvec)] \; ,
\end{equation}

\begin{equation}
    \label{eq:eqapp1-14}
    E_{\mathbb{D}_{\text{test}}} = \E_{(\xvec,\yvec) \in \mathbb{D}_{\text{test}}}[\ell(f(\xvec; \bm{\theta}), \yvec)] \; .
\end{equation}

Eq.\ref{eq:eqapp1-13} and Eq.\ref{eq:eqapp1-14} are referred to as the train error and the test error, respectively.

Reducing $E_{\mathbb{D}_{\text{train}}}$ does not define learning because Eq.\ref{eq:eqapp1-13} is a pure optimization problem. Moreover, the model can memorize the entire train set $\mathbb{D}_{\text{train}}$ and achieve zero error. However, learning consists in
\begin{enumerate}
    \item Reducing $E_{\mathbb{D}_{\text{train}}}$ (Eq.\ref{eq:eqapp1-13}),
    \item And reducing $E_{\mathbb{D}_{\text{test}}}$ (Eq.\ref{eq:eqapp1-14}).
\end{enumerate}
The second element gives the true meaning of learning which is to be able to perform well over unseen samples.

Machine learning promotes the idea of generalization by providing a probability framework to ensure that a learned model can generalize. This is done through the theory of generalization. Roughly speaking, the idea that makes the generalization possible is that
\begin{equation}
    \label{eq:eq0-15}
    E_{\mathbb{D}_{\text{test}}} \approx E_{\mathbb{D}_{\text{train}}} \; .
\end{equation}
\noindent This is correct under the assumption about the data that the samples are i.i.d.. Eq.\ref{eq:eq0-15} states that the generalization error over unseen samples can be approximated by the error over the train set. This is the actual reason to minimize the train error (Eq.\ref{eq:eqapp1-13}) and which makes the learning possible.

Before we present the theoretical guarantee of the generalization, we need to introduce introduce two concepts: growth function and Vapnik–Chervonenkis dimension (VC-dimension) \cite{vapnik1971}.

The grouth function is defined as \cite{Mohri2012bookML}

\begin{mydef}
	\label{def:defapp1-0}
	\textbf{Growth function} \\
	The growth function $\Pi_{\mathbb{H}}: \N \to \N$ for a hypothesis set $\mathbb{H}$ is defined by
	\begin{equation}
		\label{eq:eqapp1-15-1}
		\forall m \in \N, \quad \Pi_{\mathbb{H}}(m) = \max_{\{x_1, \cdots, x_m\} \subseteq \X}  \bigl|\{(h(x_1), \cdots, h(x_m)): h \in \mathbb{H}\}\bigr| \; .
	\end{equation}
\end{mydef}
\noindent Thus, $\Pi_{\mathbb{H}}(m)$ is the maximum number of distinct ways in which $m$ points can be classified using hypotheses in $\mathbb{H}$. This provides another measure of the richness of the hypothesis set $\mathbb{H}$. However, this measure does not depend on the data distribution, it is purely combinatorial.

Now, let us define the concepts of dichotomy and shattering \cite{Mohri2012bookML}. Given a hypothesis set $\mathbb{H}$, a dichotomy of a set $\mathbb{S}$ is one of the possible ways of labeling the points of $\mathbb{S}$ using a hypothesis in $\mathbb{H}$. A set $\mathbb{S}$ of $m \geq 1$ points is said to be shattered by a hypothesis set $\mathbb{H}$ when $\mathbb{H}$ realizes all possible dichotomies of $\mathbb{S}$, that is when $\Pi_H(m) = 2^m$.

The VC-dimension is defined as follows \cite{Mohri2012bookML}
\begin{mydef}
	\label{def:defapp1-1}
	\textbf{VC-dimension}\\
	The VC-dimension of a hypothesis set $\mathbb{H}$ is the size of the largest set that can be fully shattered by $\mathbb{H}$:
	\begin{equation}
		\label{eq:eqapp1-15-2}
		VCdim(\mathbb{H}) = \max\{m: \Pi_{\mathbb{H}}(m) = 2^m\} \; .
	\end{equation}
\end{mydef}

The VC-dimension $d$ measures the capacity or the complexity of
the model. In the context of classification, it is defined as the largest number of points that can be classified by the model without error. For instance, the complexity of neural network model depends on the number of hidden layers and the number of neurons. The complexity of $k$-nearest neighbor classifier depends on the number $k$. The more complex the model is, the larger space of possible functions $\mathbb{F}$. In the case of parametrized models, the capacity of a model can be indicated by the number of parameters \cite{Mohri2012bookML}. Models with large number of parameters have a large capacity.

The generalization bound using the VC-dimension is given as follows \cite{Mohri2012bookML}
\begin{mycor}
	\label{cor:corappr1-0}
	\textbf{VC-dimension generalization bounds} \\
	Let $\mathbb{H}$ be a family of functions taking values in $\{-1, +1\}$ with VC-dimension $d$. Then, for any $\delta > 0$, with probability at least $1 - \delta$, the following holds for all $h \in \mathbb{H}$
	\begin{equation}
		\label{eq:eqapp1-15-3}
		R(h) \leq \hat{R}(h) + \sqrt{\frac{2d \log \frac{em}{d}}{m}} + \sqrt{\frac{\log \frac{1}{\delta}}{2m}} \; .
	\end{equation}
\end{mycor}
\noindent Thus, the form of this generalization bound is
\begin{equation}
	\label{eq:eqapp1-15-4}
	R(h) \leq \hat{R}(h) + O\Bigg(\sqrt{\frac{\log (m/d)}{(m/d)}}\Bigg) \; ,
\end{equation}
\noindent which emphasizes the importance of the ratio $m/d$ for generalization. The theorem provides another instance of Occam's razor principle where simplicity is measured in terms of smaller VC-dimension.

When $d$ is high, which means that model has a large capacity compared to the available training samples, the test error is much higher than the train error which is referred to as \emph{overfitting} which is discussed below.

Eq.\ref{eq:eqapp1-15-3} tells us that in order to choose a better model $f$ among all the possible functions $\mathbb{F}$, one needs to strike a balance between the generalization and the complexity of the model. Simple model may fail to approximate the train data and ends up with high train error. In the other side, complex model may fail to generalize well because the large complexity term in Eq.\ref{eq:eqapp1-15-3}.

Moreover, Eq.\ref{eq:eqapp1-15-3} showed that controlling the capacity of a model is an important factor to determine the quality of the generalization. Underfitting occurs when the model is unable to obtain lower error over the train set. Overfitting occurs when there is a large gap between the train and test errors. Both behaviors can be control by altering the capacity of the model. Models with low capacity may find difficulties to fit the train set while models with high capacity can overfit by memorizing patterns in the train set that do not serve to generalize. 

One way to control the capacity of a model $f$ is by constraining its hypothesis space $\mathbb{F}$, i.e., the set of functions that the learning algorithm is allowed to select as a solution. This provides us a simple definition of the regularization in order to prevent overfitting.

\textbf{Illustration of the Issue of Overfitting:}
\bigskip

In order to show the issue of overfitting we consider a linear regression problem using a polynomial. The capacity of the polynomial can be changed by changing its degree. We refer to the set of parameters by $\bm{w}$ which is a vector containing all the coefficients of the polynomial. We use the following models for a polynomial with degree 1 (Eq.\ref{eq:eqapp1-17}), 2 (Eq.\ref{eq:eqapp1-18}) and 9 (Eq.\ref{eq:eqapp1-19}) as follows
\begin{align}
    \hat{y} &= b + w x \label{eq:eqapp1-17}\; , \\
		\hat{y} &= b + w_1 x + w_2 x^2 \label{eq:eqapp1-18} \; , \\
		\hat{y} &= b + \sum_{i=1}^9 w_i x^i \label{eq:eqapp1-19} \; . 
\end{align}

\noindent Fig.\ref{fig:figapp1-2} compares a linear (Eq.\ref{eq:eqapp1-17}), quadratic (Eq.\ref{eq:eqapp1-18}) and degree-9 polynomial (Eq.\ref{eq:eqapp1-19}) in attempt to fit a problem where the true underlying function is quadratic. The linear function is incapable to capture the curvature of the data, so it underfits. While the degree-9 function is capable of fitting the exact data, but it is also capable of representing infinitely many other functions that pass exactly through the data because the model has more parameters than the number of data which allows it to memorize the entire data. The degree-9 model succeeded to fit perfectly the train samples however it fails to extract the underlying structure of the data depicted by a curvature which is important from the generalization perspective because it shows the tendency of the data distribution. For instance, the degree-9 provides a structure with a deep valley in the left which does not appear in the true underlying function. Therefore, when predicting $\hat{y}$ of a new unseen samples in this area, the degree-9 will have a large error compared to the simple linear function. Therefore, one can see that there is a relation between the capacity of the model and the generalization error. In practice, we have a little chance to choose the optimum complexity of the model which generalizes better when there are many possible choices. In this example, the quadratic function matches perfectly the true structure of data, therefore, it generalizes better. The issue of overfitting in high capacity models can be reduced through regularization as we will see later (Fig.\ref{fig:figapp1-5}) where we \quotes{push} the optimization algorithm to \quotes{favor} a certain type of solutions over others.

\begin{figure}[!htbp]
  \centering
  \includegraphics[scale=0.2]{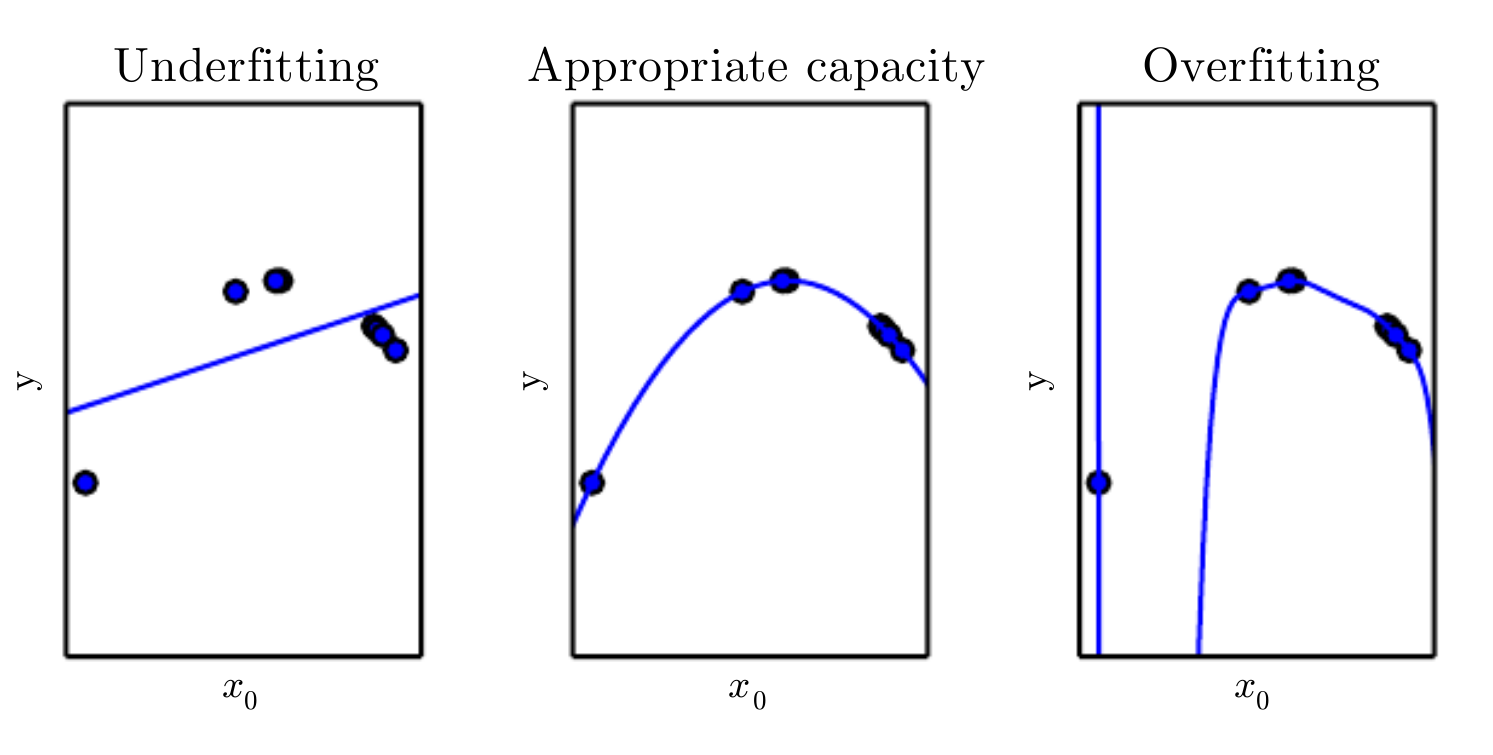}
  \caption[\bel{Model complexity and overfitting.}]{Fitting synthetic data (generated using quadratic function) using three different models: (left) linear model (Eq.\ref{eq:eqapp1-17}). middle: quadratic model (Eq.\ref{eq:eqapp1-18}). Right: degree-9 model (Eq.\ref{eq:eqapp1-19}). The regression problem $f(\xvec;\bm{w}) = \bm{w} \xvec$ is solved using Moore-Penrose pseudoinverse. (Credit: \cite{Goodfellowbook2016}) }
  \label{fig:figapp1-2}
\end{figure}

The example presented above shows that it is important to choose well the model complexity that suits the data complexity. Many early philosophers invoked the idea of model selection based on the principle of parcimony that is now most widely known as Occam's razor which is Latin for law parsimony. This idea is a problem-solving strategy attributed to William of Ockham (c. 1287-1347). This principle states that among competing hypotheses that explain known observations equally well, one should choose the simplest one. This idea was formalized in the 20th century in statistical learning theory \citep{vapnik1971, Vapnik1995, Vapnik1982, Blumer1989}.

While simpler functions are more likely to generalize better, we must still choose a model complex enough to achieve law training error. Typically, training error decrease until it asymptotes to the minimum possible error value as model capacity increases. In the other hand, the generalization error has a U-shape curve as a function of the model capacity. Fig.\ref{fig:figapp1-3} shows this typical behavior. At the left end of the graph, training error and generalization error are both high which describes the underfitting regime. As we increase the model's capacity, the training error decreases, but the gap between the training error and test error increases to enter the overfitting regime where capacity is too large, above the optimal model capacity.

\begin{figure}[!htbp]
  % \centering
  % \includegraphics[scale=0.3]{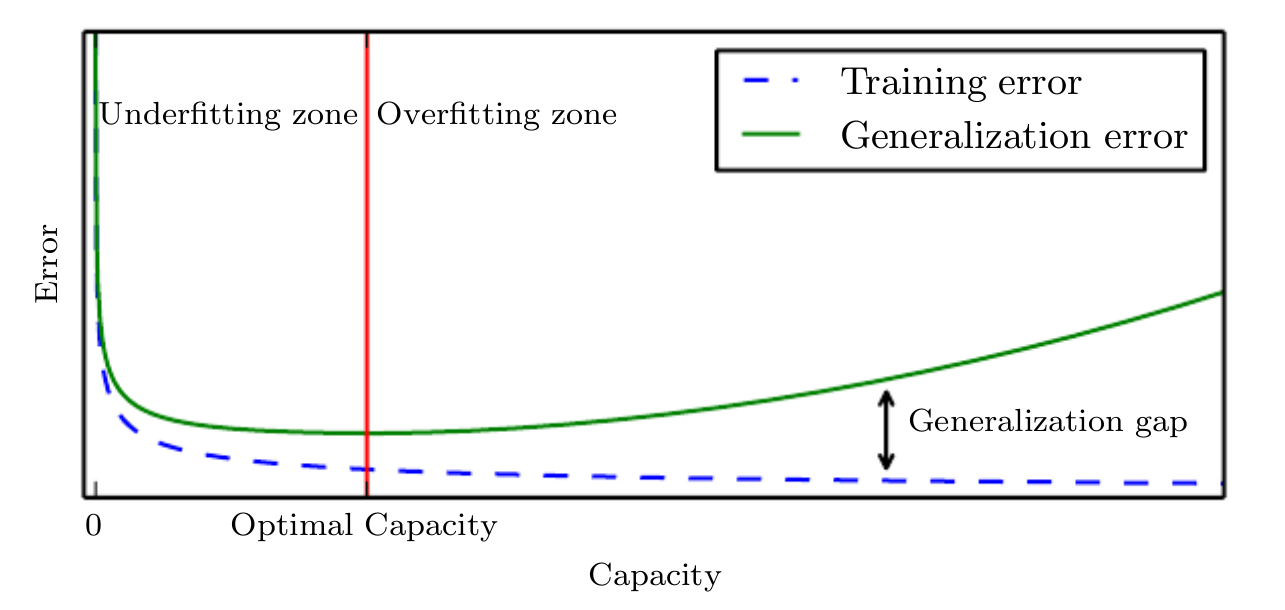}
  \begin{center}
		\input{typicalrelationcapacityandgeneralization}
	\end{center}
  \caption[\bel{Relationship between model capacity and generalization error.}]{Typical relationship between model capacity and generalization error. (Reference: \cite{Goodfellowbook2016})}
  \label{fig:figapp1-3}
\end{figure}

The overfitting can be traced back to the maximum likelihood estimation which provides us with a solution that fit exactly the data but it does not gives us the quality of the obtained solution. In other words, the MLE provides a solution that have lower error on the train data but it does not tell us how good is it to predict unseen samples. So, in the case of models with large capacity, i.e., large power to express the data (flexibility), the MLE can choose any arbitrary function that passes through the train data by putting much focus on the samples without considering the overall structure of the data. As a result, the model loses its ability to generalize well for unseen samples.

In the next section, we will present an important concept in statistics that will help us understand the relation between the model capacity and its ability to generalize to shed more light on the interest of the regularization.

\subsection{Bias-Variance Tradeoff}
\label{sub:biasvarianceapp1}

The bias-variance tradeoff is the problem of minimizing two sources of errors that prevent a model from well generalizing beyond the train data. The first error source is named the bias error which comes from erroneous assumption about the complexity of the model which means this error depends on the performance of the model in average while considering an infinite number of training samples. In the other hand, the variance error comes from the sensitivity of the model to small variations in the data. This depends on the model capacity to model the random noise (small perturbations) in the data.

The bias-variance decomposition \cite{Geman1992} provides a way to analyze the expected generalization error of a model. This decomposition gives the generalization error as a sum of two terms: the bias and the variance.

In order to formalize this decomposition, let us consider a regression problem over the distribution $p_{(\x, \y)}$. $\mathbb{D}_{\text{train}} \sim p_{(\x, \y)}$ is a sampled training data. For clearer exposition, let us take $\y = y$ to be a one-dimentional, although the results apply more generally \cite{Geman1992}. $\E[y |\xvec]$ denotes as a deterministic function that gives the value $y$ conditioned on a fixed $\xvec$. $\E[y |\xvec]$ can be seen as the best value $y$ for $\xvec$. For any function $f(\xvec)$, and any fixed $\xvec$, the regression error is \cite{Geman1992}
\begin{align}
  \E\left[(y - f(\xvec))^2|\xvec \right] & = \E\left[((y - \E[y|\xvec]) + (\E[y|\xvec] - f(\xvec)))^2 | \xvec \right] \label{eq:eqapp1-20-0}\\
  &= \E\left[(y - \E[y|\xvec])^2|\xvec \right] + (\E[y|\xvec] - f(\xvec))^2 \nonumber \\ 
    & + 2 \E \left[(y - \E[y|\xvec])|\xvec \right] \cdot (\E[y|\xvec] - f(\xvec)) \label{eq:eqapp1-20-1}\\
  &=\E\left[(y - \E[y|\xvec])^2|\xvec \right] + (\E[y|\xvec] - f(\xvec))^2 \nonumber \\ 
  &+ 2(\E[y|\xvec] - \E[y|\xvec]) \cdot (\E[y|\xvec] - f(\xvec)) \label{eq:eqapp1-20-2}\\
  & = \E\left[(y - \E[y|\xvec])^2|\xvec \right] + (\E[y|\xvec] - f(\xvec))^2 \label{eq:eqapp1-20-3} \; .
\end{align}
\noindent In other words, among all functions of $\xvec$, $f(\xvec) = \E[y|\xvec]$ is the best predictor of $y$ given $\xvec$, in the mean-squared-error.

Now, let us introduce the dependency of $f(\xvec)$ to its training sample $\mathbb{D}_{\text{train}}$ and let us note $f(\xvec; \mathbb{D}_{\text{train}})$. For clarity, we refer to $\mathbb{D}_{\text{train}}$ by $\mathbb{D}$. Now, the generalization error over a new fixed example $\xvec$ and fixed training sample $\mathbb{D}$ is computed as follows \cite{Geman1992}
\begin{align}
  \label{eq:eqapp1-20-4}
  \E\left[(y - f(\xvec; \mathbb{D}))^2 | \xvec, \mathbb{D} \right] & = \E\left[(y - \E[y|\xvec, \mathbb{D}])^2 | \xvec, \mathbb{D}\right]  + (f(\xvec; \mathbb{D}) - \E[y|\xvec])^2 \; .
\end{align}
\noindent The term ${\E\left[(y - \E[y|\xvec, \mathbb{D}])^2 | \xvec, \mathbb{D}\right]}$ does not depend on the data $\mathbb{D}$, nor on $f$. It is simply the variance of $y$ given $\xvec$. Therefore, only the term ${(f(\xvec; \mathbb{D}) - \E[y|\xvec])^2}$ measures the effectiveness of $f$ to predict $y$. The mean-squared error of $f$ as an estimator of the best prediction $\E[y|\xvec]$ is given by \cite{Geman1992}
\begin{equation}
  \label{eq:eqapp1-20-5}
  \E_{\mathbb{D}}\left[(f(\xvec; \mathbb{D}) - \E[y|\xvec])^2\right] \; ,
\end{equation}
\noindent where $\E\limits_{\mathbb{D}}$ is the expectation with respect to the training set, $\mathbb{D}$, that is the average over all possible sampled training sample $\mathbb{D}$.

The error measured in Eq.\ref{eq:eqapp1-20-5} can be further developed for any $\xvec$ as follows \cite{Geman1992}
\begin{align}
  \E_{\mathbb{D}}\left[(f(\xvec; \mathbb{D}) - \E[y|\xvec])^2\right] & = 
  \E_{\mathbb{D}}\left[( (f(\xvec; \mathbb{D}) + \E_{\mathbb{D}}[f(\xvec; \mathbb{D})]) + (\E_{\mathbb{D}}[f(\xvec; \mathbb{D})] -\E[y|\xvec]) )^2\right] \label{eq:eqapp1-20-5-1} \\
  & = \E_{\mathbb{D}}\left[(f(\xvec; \mathbb{D}) - \E_{\mathbb{D}}[f(\xvec; \mathbb{D})])^2\right] + \E_{\mathbb{D}}\left[(\E_{\mathbb{D}}[f(\xvec; \mathbb{D})] - \E[y|\xvec])^2\right] \nonumber \\ 
  &+ 2 \E_{\mathbb{D}}\left[(f(\xvec;\mathbb{D}) - \E_{\mathbb{D}}[f(\xvec; \mathbb{D})]) \cdot (\E_{\mathbb{D}}[f(\xvec;\mathbb{D})] - \E[y|\xvec]) \right]
  \label{eq:eqapp1-20-6} \\
  & = \E_{\mathbb{D}}\left[(f(\xvec; \mathbb{D}) - \E_{\mathbb{D}}[f(\xvec; \mathbb{D})])^2\right] +
  (\E_{\mathbb{D}}[f(\xvec; \mathbb{D})] - \E[y|\xvec])^2 \nonumber \\ 
  & + 2 \E_{\mathbb{D}}\left[f(\xvec;\mathbb{D}) - \E_{\mathbb{D}}[f(\xvec; \mathbb{D})]\right] \cdot (\E_{\mathbb{D}}[f(\xvec;\mathbb{D})] - \E[y|\xvec]) \label{eq:eqapp1-20-7} \\
  & = \underbrace{(\E_{\mathbb{D}}[f(\xvec; \mathbb{D})] - \E[y|\xvec])^2}_{\text{Bias}}  \nonumber \\
  & + \underbrace{\E_{\mathbb{D}}\left[(f(\xvec; \mathbb{D}) - \E_{\mathbb{D}}[f(\xvec; \mathbb{D})])^2\right]}_{\text{Variance}} \label{eq:eqapp1-20-8} \; .
\end{align}

From Eq.\ref{eq:eqapp1-20-8}, one can see that the bias is the mean error of the average models which are trained over infinite samples. Therefore, this error depends only on the model capability to model the data, i.e., model complexity. Similarly, the variance shows the capability of the model to model the variations of the data, again this is related to the complexity of the model.

As a consequence, models with small capacity will tend to have high bias because they are enable to fit well the data and low variance because they do not consider the variation in the data. In the other hand, models with high capacity will have lower bias because they can fit well the data, but they have high variance because they are sensitive to changes in the data. Hence, a tradeoff is necessary to select a model with lower bias and variance. Fig.\ref{fig:figapp1-4} shows a typical behavior of model bias and variance with respect to the model capacity. When the capacity of the model increases, the bias tends to decrease and the variance to increase yielding an U-shape of the generalization error. Above the optimum capacity, the model tends to have lower bias and higher variance. This relation is similar to the relation between the capacity, underfitting and overfitting.

\begin{figure}[!htbp]
  % \centering
  % \includegraphics[scale=0.2]{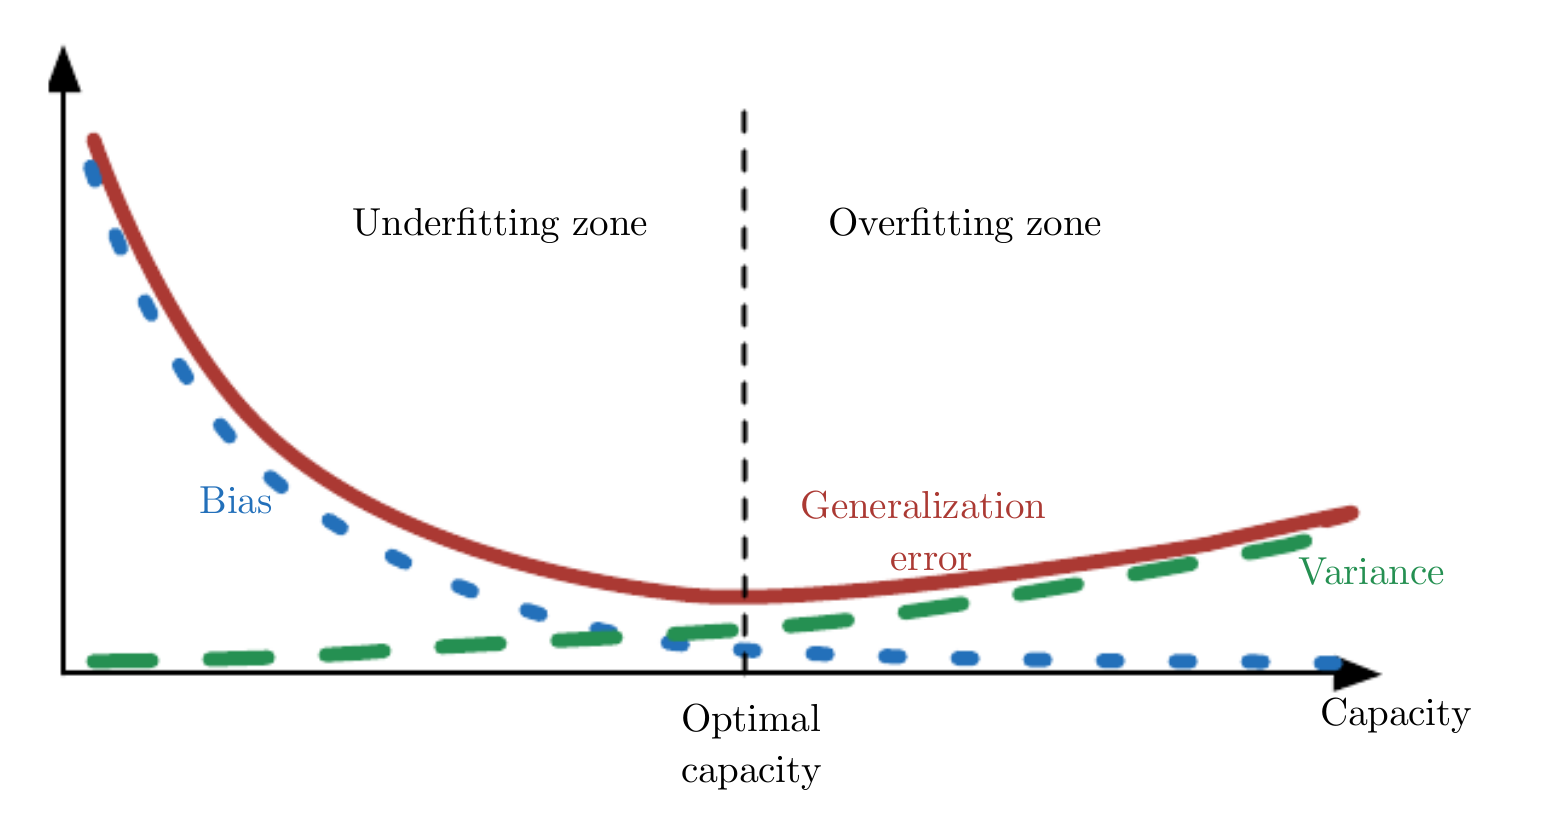}
  \begin{center}
		\input{capacitybiasvariance}
	\end{center}
  \caption[\bel{Relationship between model capacity, its bias and variance and the generalization error.}]{Typical relationship between model capacity, its bias and variance and the generalization error. (Reference: \cite{Goodfellowbook2016})}
  \label{fig:figapp1-4}
\end{figure}

When applying the regularization over a model that overfits (high capacity), we attempts to bring it from the overfitting regime toward the optimal regime by reducing its variance but without introduction significant bias.

\subsection{Regularization}
\label{sub:regularizationappapp1}

In Sec.\ref{sub:generalizationtheoryapp1}, we presented a theoretical framework of the generalization using the VC-dimension. In Sec.\ref{sub:biasvarianceapp1}, we presented the bias-variance tradeoff. It turns out that the generalization has a strong connection to the model capacity. In order the model to generalize well, it must be able to explain well the data, i.e., have a lower bias, and it has to be less sensitive to change in data, i.e., less variance. However, models with lower bias tend to have high variance and high capacity (overfitting regime) while models with lower variance tend to have high bias and low capacity (underfitting regime). In order to explain well the data, i.e. with lower bias, one needs a model with large capacity. Nonetheless,  these models tend to overfit, i.e, have a higher variance. Regularization comes to rescue overfitted models by reducing their variance and without introducing much bias, therefore, improve their generalization.

Regularization can be seen as a way of introducing some preferences or a prior of the solution of a learning problem to narrow down the hypothesis space. In a hypothesis space, there may be many solutions that reduce the bias which make them eligible solutions. However, regularization adds a preference to favor some solutions than the others. Formally, this preference can be expressed by an extra penalty to the risk functional Eq.\ref{eq:eqapp1-0}, named regularizer, to form a regularized functional as follows \cite{Goodfellowbook2016}

\begin{equation}
\label{eq:eqapp1-21}
\begin{aligned}
& \underset{\bm{\theta}}{\text{minimize}}
& & J^*_{\Omega}(\bm{\theta}) = J^*(\bm{\theta}) & \text{(Eq.\ref{eq:eqapp1-0})} \\
& \text{subject to}
& & \Omega(f) \leq c \; ,
\end{aligned}
\end{equation}
\noindent where $\Omega()$ is a function that explains the preference that we want to incorporate in the learning algorithm to condition the search space. $c$ is predefined value. This way of regularization is known as hard regularization, because it sets strict boundaries of the possible solution. It is usually used to solve conditioned problems. When ${\Omega(f) = \norm{\bm{\theta}}^2_2}$, it is known as Ivanov's method \cite{ivanov1962}.

Another form of regularization is formulated as follows
\begin{equation}
\label{eq:eqapp1-21-1}
\begin{aligned}
& \underset{\bm{\theta}}{\text{minimize}}
& & \Omega(f) & \text{(Eq.\ref{eq:eqapp1-0})} \\
& \text{subject to}
& & J^*(\bm{\theta}) \leq \delta \; ,
\end{aligned}
\end{equation}
\noindent where $\delta$ is a constant. When ${\Omega(f) = \norm{\bm{\theta}}^2_2}$, it is known as Philipp's method \cite{Phillips1962}.

Another way to regularize a model which allows the solution of unconditional optimization by weighting the regularizer as follows
\begin{equation}
    \label{eq:eqapp1-22}
    \begin{aligned}
& \underset{\bm{\theta}}{\text{minimize}}
& & J^*_{\Omega}(\bm{\theta}) = J^*(\bm{\theta}) + \lambda \Omega(f) \; ,
\end{aligned}
\end{equation}
\noindent where $\lambda > 0$ is a predefined value that regulates the regularization strength. This regularization is known as soft regularization. Functions with lower $\Omega(f)$ have more priority to be picked as a solution. Along this thesis, we will be using the soft regularization. Considering using gradient based method to optimize Eq.\ref{eq:eqapp1-22}, $\Omega()$ must be differentiable. When ${\Omega(f) = \norm{\bm{\theta}}^2_2}$, this method is known as Tikhonov's method \cite{tikhonov1963}.

It was shown in \cite{Vasin1970} that the three methods of regularization \cite{tikhonov1963, ivanov1962, Phillips1962}  are equivalent.

Expressing preferences for one function over another is a more general way to control the model's capacity. There are many ways of expressing these preferences for different solutions. In most cases, these preferences are based on our prior beliefs  about the problem in hand. Typical priors concern restrictions for smoothness in order to favor smooth functions. For instance, this can be done by penalizing the norm  of the parameters (Eq.\ref{eq:eqapp1-23}) \cite{tikhonov1963} or the norm of the function (Eq.\ref{eq:eqapp1-24}) itself or its derivatives (Eq.\ref{eq:eqapp1-25}). From a Bayesian point of view, many regularization techniques are made by imposing prior distributions on a model parameters. In some tasks, one can constrain the behavior of the function depending on some prior knowledge about the problem which is referred to by domain knowledge. This aspect of incorporating prior beliefs about the function/domain is motivated by the no free lunch theorem \cite{Wolpert1996}. Roughly speaking, this theorem states that no machine learning algorithm is universally better than any other no matter how sophisticated it is. However, this holds only when averaging over all possible data generating distribution (over all possible tasks). Therefore, if we make assumptions (priors) about the task in hand, we still have the chance to build a model that performs well on this task. Consequently, priors do matter and we should include them when designing a learning algorithm if we want our model to generalize better on this particular task. One should keep in mind  that when choosing a prior to use it as regularization, it should be intended to improve the generalization and not to reduce the bias, i.e., the training error.

\begin{equation}
    \label{eq:eqapp1-23}
    \Omega\left(f(\xvec;\bm{\theta})\right) = \norm{\bm{\theta}}_p = \left(\sum_i \magnitude{\theta_i}^p\right)^{1/p} \; .
\end{equation}

\begin{equation}
    \label{eq:eqapp1-24}
    \Omega\left(f(\xvec;\bm{\theta})\right) = \norm{f}_p = \left(\int \magnitude{f(\xvec; \bm{\theta})}^p d\xvec\right)^{1/p} \; .
\end{equation}

\begin{equation}
    \label{eq:eqapp1-25}
    \Omega\left(f(\xvec;\bm{\theta})\right) = \norm{\frac{\partial^k f(\xvec)}{\partial \xvec^k}}_p = \left(\int \magnitude{\frac{\partial^k f(\xvec; \bm{\theta})}{\partial \xvec^k} }^p d\xvec\right)^{1/p} \; .
\end{equation}
\bigskip

\textbf{Illustration of the Effect of Regularization:}
\bigskip

In order to illustrate the effect of the regularization, let us consider the problem of linear regression discussed earlier in Sec.\ref{sub:generalizationtheoryapp1}. We consider the case of the high-degree polynomial (Eq.\ref{eq:eqapp1-19}) that suffers from overfitting (Fig.\ref{fig:figapp1-2}). In order to solve this regression problem, the training criterion is modified by adding an extra penalty to regularize the model. From Fig.\ref{fig:figapp1-2}, one can see the obtained solution \quotes{oscillates} too much in order to fit exactly the data. These oscillations are mainly due to large magnitude of the estimated model. Naturally, one would prefer parameters with smaller magnitude. In order to incorporate this preference into the learning algorithm, we will be using  regularization. In this case, the regularizer consists in the square  of the $L_2$ norm (Eq.\ref{eq:eqapp1-23}, p=2) of the parameters. Therefore, the total training criterion will be
\begin{equation}
    \label{eq:eqapp1-26}
    J(\bm{w}) = \norm{y - f(\xvec; \bm{w})}_2^2 + \lambda \norm{\bm{w}}^2_2 \; ,
\end{equation}
\noindent where $\lambda$ is a value chosen before the optimization to control the strength of our preference to a solution with smaller weights. This type of regularization goes with different names such as Tikhonov regularization or weight decay. When $\lambda=0$, no preference is imposed. When $\lambda$ is large, the weights are forced to be smaller. Minimizing Eq.\ref{eq:eqapp1-26} results in a solution that makes a tradeoff between fitting the data and having weights with small magnitude. In the left of Fig.\ref{fig:figapp1-5}, the model is fitted with a large $\lambda$. This high regularization prevented the model from learning and provided a constant function. In the center of Fig.\ref{fig:figapp1-5}, a medium $\lambda$ is used which allowed the model to recover the structure of the data without passing through all the points. In the right of Fig.\ref{fig:figapp1-5} where $\lambda$ approaches zero, the non-regularized case is approached where the model overfits.

\begin{figure}[!htbp]
  \centering
  \includegraphics[scale=0.4]{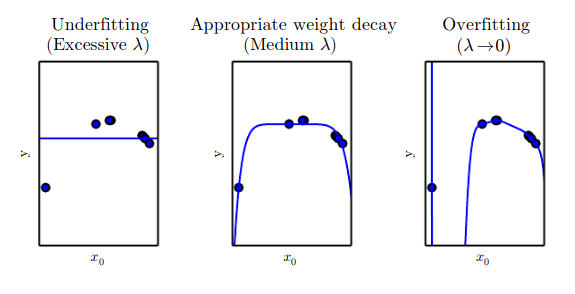}
  \caption[\bel{Impact of regularization over overfitting.}]{Fitting a degree-9 polynomial to data from Fig.\ref{fig:figapp1-2} by minimizing a regularized training criterion (Eq.\ref{eq:eqapp1-26}). (Credit: \cite{Goodfellowbook2016})}
  \label{fig:figapp1-5}
\end{figure}

By this, we close this appendix.
