# Supplementary material for: Neural Networks Regularization Through Representation Learning
Source: arXiv:1807.05292 source file (2018-07-13)
Supplement: Supplementary file 2 [file typicalrelationcapacityandgeneralization.tex]

\begin{tikzpicture}
\coordinate (center1) at (0, 0);
\coordinate (xneg) at (0, 0);
\coordinate (xpos) at (10.5, 0);
\coordinate (ypos) at (0, 5);
\coordinate (yneg) at (0, 0);

\coordinate (sge) at (0.1, 5);
\coordinate (sgem) at (3.5, 0.5);
\coordinate (ege) at (10, 2.3);

\coordinate (ste) at (0.1, 5);
\coordinate (stem) at (3.5, 0.2);
\coordinate (ete) at (10, 0.1);

\coordinate (optl) at (3.5, 0); 
\coordinate (optu) at (3.5, 5);

\coordinate (gapl) at (8, 0.2); 
\coordinate (gapu) at (8, 1.5);

\draw[->, thick] (xneg) -- (xpos) node[right] (xaxis) {\textbf{capacity}};
\draw[->, thick] (yneg) -- (ypos) node[left] (yaxis) {\textbf{error}};

\draw[color=green, ultra thick] (sge) to[out=270,in=180] (sgem) node[above, color=black]  {};
\draw[color=green, ultra thick] (sgem) to[out=0,in=200] (ege) node[above, color=black]  {\textbf{generalization error}};

\draw[color=blue, dashed, ultra thick] (ste) to[out=270,in=180] (stem) node[above, color=black]  {};
\draw[color=blue, dashed, ultra thick] (stem) to[out=-2,in=180] (ete) node[above, color=black]  {\textbf{training error}};

\draw[color=red, ultra thick] (optl) -- (optu);
\node at ($(optl) + (0mm, -3mm)$) {\textbf{optimal capacity}};
\node[text width=3cm] at ($(optu) + (20mm, -10mm)$) {\textbf{overfitting \\ zone}};
\node[text width=3cm] at ($(optu) + (-15mm, -10mm)$) {\textbf{underfitting \\ zone}};

\draw[<->, color=black, thick] (gapl) -- (gapu);
\node[right] at ($(gapu) + (0mm, -2mm)$) {\textbf{generalization gap}};

\end{tikzpicture}
