# Supplementary material for: Neural Networks Regularization Through Representation Learning
Source: arXiv:1807.05292 source file (2018-07-13)
Supplement: Supplementary file 4 [file appendix3.tex]

% ******************************* Thesis Appendix B ****************************
% Appendix A: related to the chapter "Neural networks".
\chapter{Improving Neural Networks Generalization}  %Title of the First Chapter
\label{chap:chapterapp3}

\ifpdf
    \graphicspath{{Appendix3/Figs/Raster/}{Appendix3/Figs/PDF/}{Appendix3/Figs/}}
\else
    \graphicspath{{Appendix3/Figs/Vector/}{Appendix3/Figs/}}
\fi

\makeatletter
\def\input@path{{Appendix3/}}
\makeatother

We present in this appendix other approaches used to improve the generalization performance of neural network. This includes
\begin{enumerate}
  \item technical details of the $L_2$ (Sec.\ref{sub:l2normapp3}) and $L_1$ (Sec.\ref{sub:l1normapp3}) parameters norm regularization,
  \item technical details of the early stopping as a regularization (Sec.\ref{sec:earlystoppingapp3}),
  \item noise injection (Sec.\ref{sec:noiseinjectionapp3}): to input data, to weights, and to ground-truth labels,
  \item adversarial training (Sec.\ref{sec:adversarialtrainingapp3}),
  \item and tangent propagation (Sec.\ref{sec:tangentdistanceapp3}).
  % \item and a technical presentation of pre-training technique (Sec.\ref{sec:layerwisepretrainingapp3}).
\end{enumerate}

\section[$L_p$ Parameters Norm: Technical Details]{$L_p$ Parameters Norm:  Technical Details}
\label{sec:lpnormapp3}
We provide more details on the $L_p$ parameters norm regularization for $p \in \{1, 2\}$. Let us consider the regularized training objective function
\begin{align}
    \label{eq:eqapp3-post-68}
    \widetilde{J}(\bm{\theta}; \bm{X}, \yvec) = J(\bm{\theta}; \bm{X}, \yvec) + \alpha \Omega(\bm{\theta}) ,\quad \Omega(\bm{\theta}) = \frac{1}{p} \lVert \bm{\theta} \rVert^{p}_p \; .
\end{align}

\subsection[$L_2$ Parameters Norm: Technical Details]{$L_2$ Parameters Norm:   Technical Details}
\label{sub:l2normapp3}
For $L_2$ parameters norm regularization, we have
\begin{equation}
    \label{eq:eqapp3-post-69}
    \Omega(\bm{\theta}) = \frac{1}{2} \lVert \bm{w} \rVert^2_2 \; .
\end{equation}

For the next analysis, no bias parameters are assumed, so $\bm{\theta}$ is only $\bm{w}$. Let us consider a general form of the objective function
\begin{equation}
    \label{eq:eqapp3-post-70}
    \widetilde{J}(\bm{w}; \bm{X}, \yvec) = \frac{\alpha}{2} \bm{w}^{\top} \bm{w} + J(\bm{w}; \bm{X}, \yvec) \; ,
\end{equation}
\noindent and its corresponding gradient
\begin{equation}
    \label{eq:eqapp3-post-71}
    \nabla_{\bm{w}}\widetilde{J}(\bm{w}; \bm{X}, \yvec) = \alpha \bm{w} + \nabla_{\bm{w}} J(\bm{w}; \bm{X}, \yvec) \; .
\end{equation}
\noindent Considering $\epsilon$ a learning rate, the update rule of the gradient descent at each step is performed as follows \cite{Goodfellowbook2016}

\begin{align}
    \bm{w} &\leftarrow \bm{w} - \epsilon (\alpha \bm{w} + \nabla_{\bm{w}} J(\bm{w}; \bm{X}, \yvec)) \label{eq:eqapp3-post-72-0}  \\
    \bm{w} &\leftarrow (1 - \epsilon \alpha) \bm{w} - \epsilon \nabla_{\bm{w}} J(\bm{w}; \bm{X}, \yvec) \label{eq:eqapp3-post-72} \; .
\end{align}
\noindent The last equation (Eq.\ref{eq:eqapp3-post-72}) shows that the $L_2$ regularization modifies the learning rule by multiplicatively shrinking the weight by a constant factor on each step just before performing the updates. In order to get more insights on what happens over the entire training process,  further simplification of the analysis can be made by considering a quadratic approximation of the objective function around the value of the weights that obtains minimal unregularized training cost, ${\bm{w}^* = \argmin_{\bm{w}} J(\bm{w})}$ as follows \cite{Goodfellowbook2016}
\begin{align}
    \hat{J}(\bm{w}) &= J(\bm{w}^*) + \nabla_{\bm{w}} J(\bm{w}^*)^{\top}(\bm{w} - \bm{w}^*) + \frac{1}{2} (\bm{w} - \bm{w}^*)^{\top} \bm{H} (\bm{w} - \bm{w}^*)  \label{eq:eq0-73-0} \\
    \hat{J}(\bm{w}) &= J(\bm{w}^*) + \frac{1}{2} (\bm{w} - \bm{w}^*)^{\top} \bm{H} (\bm{w} - \bm{w}^*) \label{eq:eqapp3-post-73} \; ,
\end{align}
\noindent where $\bm{H}$ is the Hessian matrix of $J$ with respect to $\bm{w}$ evaluated at $\bm{w}^*$. By definition, $\nabla_{\bm{w}}J(\bm{w}^*)=0$ at the minimum $\bm{w}^*$. Given that $\bm{w}^*$ is a local minimum, $\bm{H}$ is a positive semidefinite matrix. In order to find the analytic form of the minimum, the gradient of $\hat{J}$ is computed as follows \cite{Goodfellowbook2016}
\begin{equation}
    \label{eq:eqapp3-post-74}
    \nabla_{\bm{w}} \hat{J}(\bm{w}) = \bm{H} (\bm{w} - \bm{w}^*) \; ,
\end{equation}
\noindent and solve $\nabla_{\bm{w}} \hat{J}(\bm{w}) = 0$ for $\bm{w}$. To study the effect of the weight decay, its gradient is added to Eq.\ref{eq:eqapp3-post-74}. Now, the regularized version of $\hat{J}$ can be solved. Let $\widetilde{\bm{w}}$ denotes the location of the minimum, therefore \cite{Goodfellowbook2016}
\begin{align}
    \alpha \widetilde{\bm{w}} + \bm{H}(\widetilde{\bm{w}} - \bm{w}^*) & = 0 \label{eq:eqapp3-post-75}  \\
    (\bm{H} + \alpha \bm{I}) \widetilde{\bm{w}} & = \bm{H} \bm{w}^* \label{eq:eqapp3-post-76} \\
    \widetilde{\bm{w}} & = (\bm{H} + \alpha \bm{I})^{-1} \bm{H} \bm{w}^* \label{eq:eqapp3-post-77} \; .
\end{align}

As $\alpha$ approaches $0$, the regularized solution $\widetilde{\bm{w}}$ approaches $\bm{w}^*$. In order to have an idea on what happens when $\alpha$ grows, one can proceed using matrix decomposition. $\bm{H}$ has an eigen-decomposition using a diagonal matrix $\bm{\Lambda}$ and an orthogonal basis of eigenvectors $\bm{Q}$ such that
\begin{equation}
    \label{eq:eqapp3-post-78}
    \bm{H} = \bm{Q} \bm{\Lambda} \bm{Q}^{\top} \; .
\end{equation}
\noindent Applying this decomposition to Eq.\ref{eq:eqapp3-post-77}, the following is obtained \cite{Goodfellowbook2016}
\begin{align}
    \widetilde{\bm{w}} & = (\bm{Q} \bm{\Lambda} \bm{Q}^{\top} + \alpha \bm{I})^{-1} \bm{Q} \bm{\Lambda} \bm{Q}^{\top} \bm{w}^* \label{eq:eqapp3-post-79} \\
   \widetilde{\bm{w}} & = \left[ \bm{Q} (\bm{\Lambda} + \alpha \bm{I}) \bm{Q}^{\top}\right]^{-1} \bm{Q} \bm{\Lambda} \bm{Q}^{\top} \bm{w}^* \label{eq:eqapp3-post-80} \\
   \widetilde{\bm{w}} & = \bm{Q} (\bm{\Lambda} + \alpha \bm{I})^{-1} \bm{\Lambda} \bm{Q}^{\top} \bm{w}^* \label{eq:eqapp3-post-81-0} \\
   \underbrace{\bm{Q}^{\top} \widetilde{\bm{w}}}_{\text{Projection of } \widetilde{\bm{w}} \text{ in } \bm{Q}^{\top}} & = \underbrace{(\bm{\Lambda} + \alpha \bm{I})^{-1} \bm{\Lambda}}_{\text{Scaling factor= } \frac{\Lambda_i}{\Lambda_i + \alpha}} \underbrace{\bm{Q}^{\top} \bm{w}^*}_{\text{Projection of } \bm{w}^* \text{ in } \bm{Q}^{\top}} \label{eq:eq0-81} \; .
\end{align}
\noindent Therefore, one can see that the effect of weight decay is to rescale $\bm{w}^*$ along the axes defined by the eigenvectors $\bm{Q}^{\top}$. The components of $\bm{w}^*$ that are aligned with the $i$-th eigenvector of $\bm{H}$ are rescaled by a factor of $\frac{\Lambda_i}{\Lambda_i + \alpha}$. Therefore, in the case where $\Lambda_i \gg \alpha$, the effect of the regularization is relatively small. While, in the case where $\Lambda_i \ll \alpha$, the components of the parameters will be shrunk to have nearly zero magnitude. As a result, only directions along which the parameters contribute significantly to reducing the objective function, determined by eigenvalues with high values, are preserved relatively intact. In directions that do not contribute much in reducing the objective function, a small eigenvalue of the Hessian indicates that the movement in this direction will not significantly increase the gradient. Components of the weight vector corresponding to such unimportant directions are pushed toward zero. Fig.\ref{fig:figapp3-post-15-1} illustrates the effect of $L_2$ norm regularization on the parameters search.

\begin{figure}[!htbp]
  % \centering
  % \includegraphics[scale=0.5]{l2weightpenaltyfunction}
  \begin{center}
		\input{l2weightpenaltyfunction}
	\end{center}
  \caption[\bel{Effect of $L_2$ norm regularization.}]{Effect of $L_2$ norm regularization: it scales the weights coordinates depending on the corresponding eigenvalues.  (\emph{red contours}): indicates the $L_2$ cost ($L_2$ norm of $\bm{w}$). (\emph{green contours}): indicate the unregularized cost $J$. One contour indicates a set of parameters $\bm{w}$ that have the same cost. For instance, all the coordinates $(w_1, w_2)$ that belong to the central red circle have the same $L_2$ norm. $\bm{w}=\bm{0}$ is the optimum solution for the $L_2$ cost. $\bm{w}=\bm{w}^*$ is the minimal solution of $J$. $\bm{w}=\bm{w}^*_R$
  represents the optimum solution of the regularized cost $\widetilde{J}$ (Eq.\ref{eq:eqapp3-post-70}).(Reference: \cite{Demyanovtehsis2015})}
  \label{fig:figapp3-post-15-1}
\end{figure}

So far we have seen the effect of the weight decay over a general quadratic cost function. Using the same analysis, one can see its impact on a true quadratic function such as the linear regression
\begin{equation}
    \label{eq:eeqapp3-post-82}
    \yvec = \bm{X} \bm{w} \; .
\end{equation}
\noindent Its unregularized objective function is defined as 
\begin{equation}
    \label{eq:eqapp3-post-83}
    J(\bm{w}; \bm{X}, \yvec) = \lVert \bm{X} \bm{w} - \yvec \rVert^2_2 \; ,
\end{equation}
\noindent and its regularized objective function is defined as
\begin{equation}
    \label{eq:eqapp3-post-84}
    \widetilde{J}(\bm{w}; \bm{X}, \yvec) = \lVert \bm{X} \bm{w} - \yvec \rVert^2_2 + \alpha \lVert \bm{w} \rVert^2_2 \; .
\end{equation}
The solution for the normal equation Eq.\ref{eq:eqapp3-post-83} is given by
\begin{equation}
    \label{eq:eqapp3-post-85}
    \widetilde{\bm{w}} = (\bm{X}^{\top} \bm{X})^{-1} \bm{X}^{\top} \yvec \; ,
\end{equation}
\noindent while the solution for the regularized form is given as
\begin{equation}
    \label{eq:eqapp3-post-86}
    \widetilde{\bm{w}} = (\bm{X}^{\top} \bm{X} + \alpha \bm{I})^{-1} \bm{X}^{\top} \yvec \; .
\end{equation}

The matrix $(\bm{X}^{\top} \bm{X})$ in Eq.\ref{eq:eqapp3-post-85} is proportional to the convariance matrix $\frac{1}{m}(\bm{X}^{\top} \bm{X})$. $L_2$ norm regularization replaces this matrix by $(\bm{X}^{\top} \bm{X} + \alpha \bm{I})$ in Eq.\ref{eq:eqapp3-post-86}. The new matrix is similar to the old one but with the addition of a positive constant $\alpha$ to the diagonal. The diagonal entries in $(\bm{X}^{\top} \bm{X})$ correspond to the variance of each input feature. Therefore, $L_2$ norm regularization makes the input look like it has a high variance. This shrinks the weights on features whose covariance with the output target is low compared to the added variance. From computation perspective, $L_2$ norm regularization reduces the numerical instability of inverting $(\bm{X}^{\top} \bm{X})$ by making it non-singular. More interpretations of the $L_2$ norm regularization can be found in \cite{Boyd2004}.

\subsection[$L_1$ Parameters Norm: Technical Details]{$L_1$ Parameters Norm:  Technical Details}
\label{sub:l1normapp3}
$L_1$ parameters norm regularization is formulated as follows
\begin{equation}
    \label{eq:eqapp3-post-87}
    \Omega(\theta) = \lVert \bm{w} \rVert_1 = \sum_i |w_i| \; .
\end{equation}

While we present the $L_1$ norm regularization, we aim at highlighting the differences between $L_1$ and $L_2$ forms of regularization by considering a linear regression problem. $L_1$ weight decay controls the strength of the norm penalty by scaling $\Omega$ using a positive hyperparameter $\alpha$ as in $L_2$ norm regularization. Thus, the regularized objective function is given by 
\begin{equation}
    \label{eq:eqapp3-post-88}
    \widetilde{J}(\bm{w}; \bm{X}, \yvec) = \alpha \lVert \bm{w} \rVert_1 + J(\bm{w}; \bm{X}, \yvec)   \; ,
\end{equation}
\noindent with the corresponding gradient
\begin{equation}
    \label{eq:eqapp3-post-90}
    \nabla_{\bm{w}}\widetilde{J}(\bm{w}; \bm{X}, \yvec) = \alpha \sign(\bm{w}) + \nabla_{\bm{w}} J(\bm{w}; \bm{X}, \yvec)  \; ,
\end{equation}
\noindent where $\sign(\bm{w})$ is the sign of $\bm{w}$ applied element-wise.  Comparing $L_1$ (Eq.\ref{eq:eqapp3-post-90}) and $L_2$ (Eq.\ref{eq:eqapp3-post-71}), one can see that the $L_1$ regularization contribution is no longer scales linearly with each weight $w_i$ as in $L_2$; instead it is a constant factor with a sign equal to the sign of the parameter $w_i$.

Now, let us consider approximating the objective function around the minimum ${\bm{w}^* = \argmin_{\bm{w}} J(\bm{w})}$ by ${\hat{J}}$ using Taylor expansion. In this case, the gradient of $\hat{J}$ is computed as \cite{Goodfellowbook2016}
\begin{equation}
    \label{eq:eqapp3-post-91}
    \nabla_{\bm{w}}\hat{J}(\bm{w}) = \bm{H} (\bm{w} - \bm{w}^*) \; ,
\end{equation}
\noindent where $\bm{H}$ is the Hessian matrix of $J$ with respect to $\bm{w}$ evaluated at $\bm{w}^*$. However, this time further simplification are made by assuming that the Hessian is diagonal
\begin{equation}
    \label{eq:eqapp3-post-92}
    \bm{H} = \diag([H_{1,1}, \cdots, H_{n,n}]), \quad \forall i: H_{i,i} > 0 \; .
\end{equation}
\noindent This assumption holds if the data for the linear regression problem has been preprocessed to remove all correlation between the input features. Now, the quadratic approximation of the $L_1$ regularized objective function can be written as \cite{Goodfellowbook2016}
\begin{equation}
    \label{eq:eqapp3-post-93}
    \hat{J}(\bm{w}; \bm{X}, \yvec) = \J(\bm{w}^*; \bm{X}, \yvec) + \sum_i \left[\frac{1}{2} H_{i,i} (w_i - w^*_i)^2 + \alpha |w_i| \right] \; .
\end{equation}

Eq.\ref{eq:eqapp3-post-93} has an analytic solution for each dimension $w_i$ under the following form \cite{Goodfellowbook2016}
\begin{equation}
    \label{eq:eqapp3-post-94}
    w_i = \sign(w^*_i) \max\left\{|w^*_i| - \frac{\alpha}{H_{i,i}}, 0\right\} \; .
\end{equation}
\noindent When $w^*_i > 0$, there are two possible outcomes:
\begin{enumerate}
    \item $w^*_i \leq \frac{\alpha}{H_{i,i}}$: The optimal value of $w_i$ is simply $w_i = 0$. This occurs when the contribution of the $L_1$ regularization penalty takes over the objective function $J(\bm{w}; \bm{X}, \yvec)$. 
    \item $w^*_i > \frac{\alpha}{H_{i,i}}$: In this case, the regularization does not set the optimal value of $w_i$ to zero but instead shift it in the direction of zero by $\frac{\alpha}{H_{i,i}}$.
\end{enumerate}
\noindent In the case where $w^*_i < 0$, the $L_1$ penalty makes $w_i$ less negative by a distance $\frac{\alpha}{H_{i,i}}$ or set it to zero.

\bigskip

Comparing to $L_2$, $L_1$ regularization results in a solution where most of the parameters are zero, i.e., a sparse solution. The sparsity behavior in $L_1$ is different than the one in $L_2$ where the parameters are pushed toward zero in some cases. Eq.\ref{eq:eqapp3-post-81-0} gave the solution $\widetilde{\bm{w}}$ for $L_2$ regularization. If the same assumption, used in the case of $L_1$, is considered about the Hessian matrix, one can find that $\widetilde{w}_i = \frac{H_{i,i}}{H_{i,i} + \alpha} w^*_i$. Therefore, if $w^*_i$ is nonzero, $\widetilde{w}_i$ 
remains nonzero. This shows that $L_2$ does not promote sparse solutions, while $L_1$ regularization may set a subset of the parameters to zero for large enough $\alpha$. Fig.\ref{fig:figapp3-post-16-1} illustrates the geometric effect introduced by the $L_1$ regularization on the parameters search. This sparsity aspect plays an important role in machine learning particularly as a feature selection mechanism. Feature selection simplifies machine learning by choosing which subset of input features are relevant to predict the output target. This has a key role in application where the interpretation is highly important. For instance, when building a model to predict a disease based on set of input features, it is important to know which factors are implicated in the cause of the disease. The sparsity has been used for a long time, for instance, the well known LASSO \cite{Tibshirani94regressionshrinkage} (Least Absolute Shrinkage and Selection Operator) model integrates an $L_1$ penalty with a linear model. More details on the $L_1$ regularization and sparsity can be found in \cite{Hastie2015book}.

\begin{figure}[!htbp]
  % \centering
  % \includegraphics[scale=0.5]{l1weightpenaltyfunction}
  \begin{center}
		\input{l1weightpenaltyfunction}
	\end{center}
  \caption[\bel{Effect of $L_1$ norm regularization.}]{Effect of $L_1$ norm regularization: Large $\alpha$ makes some parameters equal to 0. (\emph{red contours}): indicate the $L_1$ cost ($L_1$ norm of $\bm{w}$). (\emph{green contours}): indicate the unregularized cost $J$. $\bm{w}=\bm{w}^*$ is the minimal solution of $J$. $\bm{w}=\bm{w}^*_R$
  represent the optimum solutions of the regularized cost $\widetilde{J}$ (Eq.\ref{eq:eqapp3-post-88}). In this example, $L_1$ regularization allows two solutions $\bm{w}^*_R$ depending on the value of $\alpha$. Small $\alpha$ results in a solution a little far from the origin. However, large $\alpha$ provides a sparse solution where $w_1= 0$. (Reference: \cite{Demyanovtehsis2015})}
  \label{fig:figapp3-post-16-1}
\end{figure}

\section[Early Stopping as a Regularization: Technical Details]{Early Stopping as a Regularization: Technical Details}
\label{sec:earlystoppingapp3}
We have mentioned in Sec.\ref{subsub:earlystopping0} that early stopping can play a role of a regularizer. Formal demonstration is provided in this section.

Consider a network with weights initialized from a distribution with zero mean. Let us see formally how early stopping can be a regularizer. Many authors \cite{bishop1995ICANN, sjoberg1995} argued that early stopping has the effect of restricting the optimization procedure to a relatively small volume of parameter space in the neighborhood of the initial parameter $\bm{\theta}_0$ (Fig.\ref{fig:figapp3-post-18}). More specifically, consider taking $\tau$ optimization steps and with a learning rate $\epsilon$. One can view $\epsilon \tau$ as the effective capacity. Restricting the number of iteration and the learning rate limits the volume of the parameter space reachable from $\bm{\theta}_0$. In this case, $\epsilon \tau$ behaves as if it was the reciprocal of the coefficient used for weight decay.

To compare early stopping with the classical $L_2$ regularization, let us consider a setting where parameters are linear weights $\bm{\theta} = \bm{w}$. One can approximate the objective function $J$ with a quadratic form in the neighborhood of the empirically optimal value of the weights $\bm{w}^*$ \cite{Goodfellowbook2016}
\begin{equation}
    \label{eq:eqapp3-post-113}
    \hat{J}(\bm{w}) = J(\bm{w}^*) + \frac{1}{2} (\bm{w} - \bm{w}^*)^{\top} \bm{H} (\bm{w} - \bm{w}^*) \; ,
\end{equation}
\noindent where $\bm{H}$ is the Hessian matrix of $J$ with respect to $\bm{w}$ evaluated at $\bm{w}^*$. This makes $\bm{H}$ positive semidefinite. The gradient of the $\hat{J}$ is
\begin{equation}
    \label{eq:eqapp3-post-114}
    \nabla_{\bm{w}} \hat{J}(\bm{w}) = \bm{H} (\bm{w} - \bm{w}^*) \; .
\end{equation}
Now, let us study the trajectory followed by the parameter vector during training. For simplicity, the initial parameters are set to the origin, $\bm{w}^{(0)} = \bm{0}$. Then, the gradient descent updates are performed as follows \cite{Goodfellowbook2016}
\begin{align}
    \bm{w}^{(\tau)} & = \bm{w}^{(\tau -1)} - \epsilon \nabla_{\bm{w}} \hat{J}(\bm{w}^{(\tau -1)} \label{eq:eqapp3-post-115} \\
    &= \bm{w}^{(\tau-1)} - \epsilon \bm{H} (\bm{w}^{(\tau -1)} - \bm{w}^*) \label{eq:eqapp3-post-116} \\
    \bm{w}^{(\tau)}- \bm{w}^* &= (\bm{I} - \epsilon \bm{H}) (\bm{w}^{(\tau -1)} - \bm{w}^*) \label{eq:eqapp3-post-117} \; .
\end{align}
\noindent Now, using the eigendecomposition of ${\bm{H}}$: ${\bm{H} = \bm{Q} \bm{\Lambda} \bm{Q}^{\top}}$, where $\bm{\Lambda}$ is a diagonal matrix and $\bm{Q}$ is an orthonormal basis of eigenvectors, it results \cite{Goodfellowbook2016}
\begin{align}
    \bm{w}^{(\tau)}- \bm{w}^* &= (\bm{I} - \epsilon \bm{Q} \bm{\Lambda} \bm{Q}^{\top}) (\bm{w}^{(\tau -1)} - \bm{w}^*) \label{eq:eqapp3-post-118} \\
    \bm{Q}(\bm{w}^{(\tau)}- \bm{w}^*) &= (\bm{I} - \epsilon \bm{\Lambda})\bm{Q}^{\top} (\bm{w}^{(\tau -1)} - \bm{w}^*) \; . \label{eq:eqapp3-post-119}
\end{align}
\noindent Assuming that $\epsilon$ is chosen to be small enough to grantee ${|1 - \epsilon \lambda_i|< 1}$, it can be shown \cite{bishop1995ICANN, Goodfellowbook2016} that the parameter trajectory during training after $\tau$ parameter updates has the following form
\begin{equation}
    \label{eq:eqapp3-post-120}
    \bm{Q}^{\top} \bm{w}^{(\tau)} = \left[\bm{I} - (\bm{I} - \epsilon\Lambda)^{\tau}\right] \bm{Q}^{\top} \bm{w}^* \; .
\end{equation}
\noindent Eq.\ref{eq:eqapp3-post-81-0} can be rearranged as
\begin{equation}
    \label{eq:eqapp3-post-121}
    \bm{Q}^{\top} \widetilde{\bm{w}} = \left[ \bm{I} - (\Lambda + \alpha \bm{I}) ^{-1} \alpha \right] \bm{Q}^{\top} \bm{w}^* \; .
\end{equation}
\noindent Comparing Eq.\ref{eq:eqapp3-post-120} and Eq.\ref{eq:eqapp3-post-121}, one can see that if $\epsilon$, $\alpha$ and $\tau$ are chosen such that \cite{bishop1995ICANN, Goodfellowbook2016}
\begin{equation}
    \label{eq:eqapp3-post-122}
    (\bm{I} - \epsilon\Lambda)^{\tau} = (\Lambda + \alpha \bm{I}) ^{-1} \alpha \; ,
\end{equation}
\noindent then $L_2$ regularization and early stopping can be seen as equivalent (under the quadratic approximation and the previous stated assumptions). Going further, by approximating both sides of Eq.\ref{eq:eqapp3-post-122}, one can conclude that if all $\lambda_i$  are small, then \cite{bishop1995ICANN, Goodfellowbook2016}
\begin{align}
    \tau \approx \frac{1}{\epsilon \alpha} \label{eq:eqapp3-post-123} \; , \\
    \alpha \approx \frac{1}{\tau \epsilon} \label{eq:eqapp3-post-124} \; .
\end{align}
\noindent Thus, under these assumptions, the number of training iterations $\tau$ plays a role inversely proportional to the $L_2$ regularization parameter, and the inverse of $\tau \epsilon$ plays the role of the weight decay. Therefore, the parameter corresponding to the directions of significant curvature of the objective function are regularized less than directions of less curvature. In the context of early stopping, this means that parameters that correspond to directions of significant curvature tend to learn early relatively to parameters corresponding to directions of less curvature. This is actually very intuitive. Parameters that correspond to high curvature tend to learn faster, which means, that in a short time, they have already learned something. While given the same amount of time, parameters that correspond to low curvature will tend to learn slowly. Therefore, early stopping mimics $L_2$ regularization by repressing parameters corresponding to low curvature and preventing parameter corresponding to high curvature to significantly grow. One can note that early stopping has the advantage to be determined through one run of the training process while $L_2$ regularization requires many runs with different values.
\begin{figure}[!htbp]
  % \centering
  % \includegraphics[scale=0.4]{earlystoppingasl2regu}
  \begin{center}
		\input{earlystoppingasl2regu}
	\end{center}
  \caption[\bel{An illustration of the effect of early stopping.}]{An illustration of the effect of early stopping. (\emph{green contours}): indicate the contours the unregularized cost $J$ (no early stopping). (\emph{red dashed contours}): indicate the contours of the $L_2$ cost, which cause the minimum of the total cost to lie nearer the origin rather the minimum of the unregularized cost. (\emph{gray dotted path}): indicates the trajectory taken by the SGD starting from the origin. Rather than stopping at the optimum point $\bm{w}^*$ that minimizes the cost, early stopping results in the trajectory stopping at an earlier point $\widetilde{\bm{w}}$.  (Credit: \cite{bishop1995ICANN, Goodfellowbook2016})}
  \label{fig:figapp3-post-18}
\end{figure}

\section{Noise Injection}
\label{sec:noiseinjectionapp3}
We discuss here three types of injected noise depending on the element receiving the noise: the input data, the parameters, and the ground-truth labels. Adding noise to the hidden units will be discussed later.

\subsection{Noise Injection to Input Data \texorpdfstring{$\xvec$}{x}}
\label{sub:injectnoiseintodataapp3}
In Sec.\ref{sub:dataaugmentation0}, we motivated the use of noise to the input data as a data augmentation. The type of noise might be different, but when adding Gaussian noise, it can be shown \cite{Bishop1995} that it is equivalent to Tikhonov regularization \cite{tikhonov77}. 

In order to check the impact of adding noise  to the input samples over the cost function, let us consider the following setup. Let
\begin{equation}
    \label{eq:eqapp3-95}
    \ell(f(\xvec), y) = \lVert y - f(\xvec) \rVert^2_2 \; ,
\end{equation}
\noindent be the mean squared error for one single pair $(\xvec, y)$. The added noise $\bm{\epsilon}_{\xvec}$ is a Gaussian noise: ${\bm{\epsilon}_{\xvec} \sim P_{\xvec} = \mathcal{N}(0, \sigma^2\bm{I})}$. It modifies the cost function as follows \cite{tikhonov77, Demyanovtehsis2015}
\begin{equation}
    \label{eq:eqapp3-96}
    \ell_{\epsilon_{\xvec}}(f(\xvec), y) = \E_{\mathbf{\epsilon} \sim P_{\xvec}}\left[(y - f(\xvec + \bm{\epsilon}_{\xvec}))^2\right] \; .
\end{equation}
\noindent Using Taylor approximation around $\xvec$
\begin{equation}
    \label{eq:eqapp3-97}
    f(\xvec + \bm{\epsilon}_{\xvec}) \approx f(\xvec) + \nabla_{\xvec} f(\xvec) \cdot \epsilon_{\xvec}^{\top} \; ,
\end{equation}
\noindent where ($\cdot$) is the dot product. $\ell_{\bm{\epsilon}_{\xvec}}$ (Eq.\ref{eq:eqapp3-96}) can be derived as \cite{tikhonov77, Demyanovtehsis2015}
\begin{align}
    \ell_{\bm{\epsilon}_{\xvec}} &\approx \E_{\bm{\epsilon} \sim P_{\xvec}}\left[(y - f(\xvec) - \nabla_{\xvec} f(\xvec) \cdot \epsilon_{\xvec}^{\top} )^2\right] \label{eq:eqapp3-98} \\
    & = \E_{\bm{\epsilon} \sim P_{\xvec}}\left[ (y - f(\xvec))^2 + (\nabla_{\xvec} f(\xvec)\cdot \epsilon_{\xvec})^2 - 2 (y - f(\xvec)) \nabla_{\xvec} f(\xvec) \cdot \epsilon_{\xvec}^{\top}\right] \label{eq:eqapp3-99} \\
    & = (y - f(\xvec))^2 + \E_{\bm{\epsilon} \sim P_{\xvec}}\left[ \bm{\epsilon}_{\xvec} \nabla_{\xvec} f(\xvec)^{\top} \nabla_{\xvec} f(\xvec) \bm{\epsilon}_{\xvec}^{\top}\right] - 2 (y - f(\xvec)) \nabla_{\xvec} f(\xvec) \cdot \E_{\bm{\epsilon} \sim P_{\xvec}}\left[\bm{\epsilon}_{\xvec}^{\top}\right] \label{eq:eqapp3-100}\\
    & = (y - f(\xvec))^2 + \sigma^2 \Tr(\nabla_{\xvec} f(\xvec)^{\top} \nabla_{\xvec} f(\xvec)) \label{eq:eqapp3-101} \\
    & = l(y, f(\xvec))  + \underbrace{\sigma^2 \lVert \nabla_{\xvec} f(\xvec) \rVert^2_2}_{\text{Regularization penalty}} \label{eq:eqapp3-102}
\end{align}
\noindent Therefore, the regularization term over the whole training sample $\mathbb{D}$ with size $N$ is equivalent to
\begin{equation}
    \label{eq:eq0-103}
    \Omega(f(\xvec; \mathbb{D})) = \frac{\sigma^2}{N} \sum^N_{i=1} \lVert \nabla_{\xvec} f(\xvec_i)\rVert^2_2 \;, \quad (\xvec_i, y_i) \in \mathbb{D} \; . 
\end{equation}
\noindent Therefore, adding Gaussian noise to the input samples requires the algorithm to have small derivatives of the output with respect to the input $x$. This means that the output becomes more robust to the variations in the input. This invariance is widely desirable in machine learning applications.

\subsection{Noise Injection to Weights \texorpdfstring{$\bm{w}$}{w}}
\label{sub:injectiontoweightsapp3}
Another way where adding noise can be helpful in regularizing the model is by adding random noise to the weights. The approach has been applied primarily with recurrent neural networks \cite{jim1996analysis, NIPS2011}. It can be interpreted as a stochastic implementation of Bayesian inference over the weights. This considers the weights as uncertain and therefore they are represented by a probability distribution that reflects this uncertainty. Adding noise to the weights is a practical way to reflect this uncertainty.

Assuming the Gaussian noise: ${\bm{\epsilon}_{\bm{w}} \sim P_{\bm{w}} = \mathcal{N}(0, \sigma^2\bm{I})}$ and using the approximation 
\begin{equation}
    \label{eq:eqapp3-104}
    f(\xvec; \bm{w} + \bm{\epsilon}_{\bm{w}}) \approx f(\xvec; \bm{w}) + \nabla_{\bm{w}} f(\xvec; \bm{w}) \cdot \bm{\epsilon}_{\bm{w}} \; ,
\end{equation}
\noindent the same derivations as in Eq.\ref{eq:eqapp3-102} can be performed to obtain
\begin{equation}
    \label{eq:eqapp3-105}
    \ell_{\bm{\epsilon}_{\bm{w}}} \approx \ell(f(\xvec), y) + \sigma^2 \lVert \nabla_{\bm{w}} f(\xvec; \bm{w})\rVert^2_2 \; .
\end{equation}

This form of regularization encourages the parameters to go to regions of parameters space where small perturbations of the weights have relatively small influence on the output. In other words, it pushes the models weights to regions where the model is relatively insensitive to small variations in the weights by finding weights that are not merely minima, but minima surrounded by flat regions \cite{Hochreiter95simplifyingneural}. In the case of regression where ${f(\xvec; \bm{w}) = \bm{w}^{\top} \xvec + b}$, this regularization term collapses into
\begin{equation}
    \label{eq:eqapp3-106}
    \Omega(f(\xvec; \mathbb{D})) = \sigma^2 \E_{\x}\left[\lVert \xvec \rVert^2_2\right] \; ,
\end{equation}
\noindent which is not a function of the parameters, therefore, it has no impact on the gradient $\nabla_{\bm{w}}\ell_{\bm{\epsilon}_{\bm{w}}}$.

\subsection{Noise Injection to Ground-truth Labels \texorpdfstring{$\yvec$}{y}}
\label{sub:injectiontoyapp3}
Nowadays, training datasets are becoming large. This often leads to have unreliable labels such as those obtained from Amazon's Mechanical Turk or social media platforms. Maximizing $\log p(\y|\x; \bm{w})$ when $\bm{y}$ is wrong can lead to poor performance. For instance, in the case of classification task with $K$ classes, one can assume that every label $\bm{y}$ of the ground-truth is correct with certainty $1 - \epsilon$, otherwise it may be the other possible labels by certainty of $\frac{\epsilon}{K-1}$.

Label smoothing regularization goes in the same direction by introducing noise into the labels $\yvec$ for the classification task. For each training sample $\xvec$, the model computes the probability of each label $k$ as
\begin{equation}
    \label{eq:eqapp3-107}
    P(k|\xvec) = \frac{\exp(z_k)}{\sum^K_{i=1}z_i} \; , \quad \text{for } k \in \{1, \cdots, K\} \; ,
\end{equation}
\noindent where $z_k$ are the linear output of the output layer. Let us consider the ground-truth distribution over the labels $\yvec$ of each sample $\xvec$
\begin{equation}
    \label{eq:eqapp3-108}
    q(k|\xvec) = \delta_{k, y} \; ,
\end{equation}
\noindent Where $\delta_{k, y}$ is the Kronecker delta. This forms a probability distribution: ${\sum^K_{k=1} q(k|\xvec) = 1}$.

Let us define the loss function for each example as the loss entropy
\begin{equation}
    \label{eq:eqapp3-109}
    l(\xvec,\yvec) = -\sum^K_{k=1} \log(P(k|\xvec)) q(k|\xvec) \; ,
\end{equation}
\noindent which has a simple gradient form (Eq.\ref{eq:eqapp2-65})
\begin{equation}
    \label{eq:eqapp3-110}
    \frac{\partial l}{\partial z_k} = P(k) - q(k) \;,
\end{equation}
\noindent which is bounded between $-1$ and $1$.

Using the label distribution $q(k|\xvec)$ in Eq.\ref{eq:eqapp3-108}, as it is, can cause some issues. Maximum likelihood learning with softmax classifier and hard targets (Eq.\ref{eq:eqapp3-108}) may actually never converge. In other words, the softmax will never predict a probability with exactly $0$ or exactly $1$. Therefore, it will continue to learn and make the weights large and large. Increasing the logits $z_k$ indefinitely to fit the target $y$ can cause two issues. First, it may result in an overfitting. If the model learns to assign a full probability to the ground-truth label for each training example, there is no guarantee that the model is capable of generalization. Second, it encourages the differences between the largest logit and all other logits to become large, and this combined with the bounded gradient $\frac{\partial l}{\partial z_k}$, reduces the ability of the model to adapt to new situations. This happens because the model becomes too confident about its prediction. Label smoothing was proposed \cite{SzegedyVISW16CVPR, PereyraTCKH17CORR, Jindal2016IDM} in order to encourage the model to be less confident which regularizes it and makes it more adaptable. Intuitively, this may be seen as an introduction to some suspicion in the model decision in order to avoid taking quick and more confident decisions. The method consists in considering a distribution $u(k)$ over the labels, independent of the training samples $\xvec$, and a smoothing parameter $\epsilon$. For a training example with ground-truth label $\yvec$, we replace the label distribution $q(k|\xvec)$ in Eq.\ref{eq:eqapp3-108} with
\begin{equation}
    \label{eq:eqapp3-111}
    q^{\prime}(k|\xvec) = (1 - \epsilon) \delta_{k, y} + \epsilon u(k) \; .
\end{equation}
\noindent In practice, $u(k)$ can be the uniform distribution
\begin{equation}
    \label{eq:eq0-112}
    u(k) = \frac{1}{K} \;.
\end{equation}
\noindent Therefore, the new label distribution ${q^{\prime}(k|\xvec)}$ will assign a probability of ${(1-\epsilon) + \frac{\epsilon}{K}}$ to the correct label and ${\frac{\epsilon}{K}}$ to the everything else.

Using label smoothing as a regularization has shown to improve the performance  \cite{SzegedyVISW16CVPR, PereyraTCKH17CORR, Jindal2016IDM}.

\section{Adversarial Training}
\label{sec:adversarialtrainingapp3}

Neural networks have begun to reach human performance on many tasks when evaluated on an i.i.d. test set. Naturally, one wonders if truly these models have reached the human performance. To check this, one can search for examples that the model misclassifies. One should keep in mind that there is a still large difference between human and machine understanding such the case in image perception. \cite{SzegedyZSBEGF13CORR} discovered an interesting phenomena: neural networks that perform at human level accuracy can have nearly $100\%$ error rate on examples that are intentionally constructed by using an optimization procedure to search for an input $\xvec^{\prime}$, referred to as adversarial example, near a data point $\xvec$ such that the model output is very different at $\xvec$. In many cases, $\xvec^{\prime}$ can be so similar to $\xvec$ that a human observer can not tell the difference between the original example and the adversarial example, however, the model can make highly different prediction (Fig.\ref{fig:figapp3-19}).

\begin{figure}[!htbp]
    \vspace{-.05in}
    \centering
% m columns to vertically center the text
% using m requires that I specify the width
% m seems to only successfully vertically center if I make *all* columns m
% m left aligns, so I need to use >{\centering\arraybackslash} before the m
% to get horizontal center alignment
\begin{tabular}{>{\centering\arraybackslash}m{.2\textwidth}m{.5in}>{\centering\arraybackslash}m{.2\textwidth}m{.1in}>{\centering\arraybackslash}m{.2\textwidth}}
    \centering\arraybackslash
%abs max for panda was 138, eps was 1., so relative eps is ~.007
    \includegraphics[width=.2\textwidth]{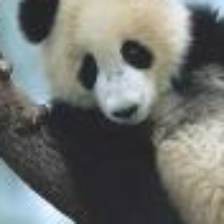} &%
    \centering\arraybackslash%
$\ +\ .007\ \times$ &%
    \includegraphics[width=.2\textwidth]{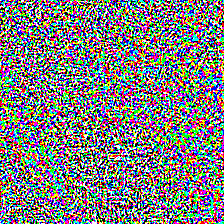} &%
    $=$ & %
    \includegraphics[width=.2\textwidth]{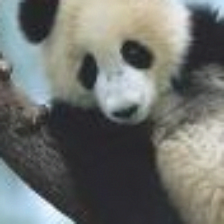} \\
    $\centering \vx$     &%
    & $\sign (\nabla_\vx J(\vtheta, \vx, y) )$ & & $\vx + \epsilon \sign (\nabla_\vx J(\vtheta, \vx, y) )$ \\
    ``panda'' &                & ``nematode''     &   & ``gibbon'' \\
    57.7\% confidence &        &   8.2\% confidence & & 99.3 \% confidence
\end{tabular}
    \caption[Fast adversarial sample generation.]{
    A demonstration of fast adversarial example generation applied to GoogLeNet
    \cite{szegedyLJSRAEVR14}
    on ImageNet.
    By adding an imperceptibly small vector whose elements are equal to the sign of the elements
    of the gradient of the cost function with respect to the input, we can
    change GoogLeNet's classification of the image.  (Credit: \cite{GoodfellowSS14CORR})
    }
\label{fig:figapp3-19}
\end{figure}

\cite{SzegedyZSBEGF13CORR} proposed a box-constrained optimization problem using L-BFGS \cite{Liu1989}. For a given $\xvec \in \R^m$ image, and target label $l \in \{1, \cdots, k\}$, solve the following problem
\begin{equation}
\begin{aligned}
& \underset{\xvec}{\text{minimize}}
& & \lVert \bm{r} \rVert_2 \\
& \text{subject to}
& & f(\xvec + \bm{r}) = l \text{ and } \xvec + \bm{r} \in [0, 1]^m \; .
\end{aligned}
\label{eq:eq0-145}
\end{equation}
\noindent Other than the trivial solution, $\bm{r}=\bm{0}$ so ${\xvec} = \xvec^{\prime}$ with the same true label, there exist other solutions in the neighborhood of the original input that have different labels. \cite{SzegedyZSBEGF13CORR} found that adversarial examples are the same for networks trained with different initialization parameters, and on a subset of the training set. Therefore, the authors concluded that this behavior is not the result of overfitting but rather a universal issue in neural network.
\bigskip

\cite{GoodfellowSS14CORR} argued that the primary cause of these adversarial examples is excessive linearity. Neural networks are built out of primarily linear building blocks. In some experiments the overall function they implemented proved to be highly linear as a result. In some cases, the linearity or close to linearity is introduced to the network on purpose for ease the optimization \cite{JarrettKRL09ICCV, NairHicml10, AISTATS2011GlorotBB11}. Unfortunately, the value of linear function can change very rapidly if it has a high dimension input. If we change each input by $\epsilon$, then the linear function with weight $\bm{w}$ can change by as much as ${\epsilon \lVert\bm{w}\rVert_1}$, which can be very large amount when $\bm{w}$ is high dimensional. This can be easily shown using a linear model and considering the direction of the added perturbation as $\sign(\bm{w})$. Using adversarial training discourages this highly sensitive locally linear behavior by encouraging the network to be locally constant in the neighborhood of the training data. Let consider the gradient of the loss function with respect to the input vector ${\nabla_{\xvec} J(\xvec)}$. If $\epsilon$ is small, one can assume that  \cite{Goodfellowbook2016}
\begin{equation}
    \label{eq:eqapp3-146}
    \xvec^{\prime} = \xvec + \epsilon \sign(\nabla_{\xvec} J(\xvec)) \; ,
\end{equation}
\noindent will be close to $\xvec$, and will have the same label. If ${\xvec \in \R^m}$, then the value of the loss function for the new sample will be \cite{Goodfellowbook2016}
\begin{align}
    J(\xvec^{\prime}) & \approx J(\xvec) + \epsilon \sign(\nabla_{\xvec} J(\xvec)) \cdot \nabla_{\xvec} J(\xvec)^{\top} \label{eq:eqapp3-147} \\
    & = J(\xvec) + \epsilon \lVert \nabla_{\xvec} J(\xvec) \rVert_1 \label{eq:eqapp3-148} \\
    & = J(\xvec) + \epsilon m \zeta \label{eq:eqapp3-149} \; ,
\end{align}
\noindent where $\zeta$ is the average magnitude of ${\lVert \nabla_{\xvec} J(\xvec) \rVert_1}$: ${\zeta = \frac{1}{m} \lVert \nabla_{\xvec} J(\xvec) \rVert_1}$. The larger $m$, the quicker $J(\xvec)$ grows in this direction. In the image classification task, $m$ is the number of pixels, which may be very large. At the same time, the parameter $\epsilon$ may be chosen to be less than $\frac{1}{255}$, which guarantees that the modified image $\xvec^{\prime}$ will be perceptually the same as the original image $\xvec$. 

\cite{FawziCONF2015} came up to similar conclusion about the cause of adversarial examples. \cite{FawziCONF2015} argued that such examples appear in high dimensional space for the classifiers that are not flexible enough, and therefore appear not only in neural networks. The authors demonstrated that this issue is uncorrelated with the robustness to random noise.

Adversarial examples have many implications in many applications. For instance, computer security where the aim is to provide tools to protect algorithms against adversarial attacks. However, this subject is out of the scope of this thesis. Instead, we tackle adversarial examples as a regularization technique to improve the model generalization.
\bigskip

In most classification tasks, class probability are supposed to be continuous with respect to the input vector. Therefore, all objects within small neighborhood of each training sample should have the same label as this sample. This referred to as the manifold assumption \cite{Chapelle2010semisupervisedl}. Adversarial examples showed that this assumption is not systematically learned by a neural network. As a consequence, it has to be incorporated into the network manually during learning using a regularization method. One of the straightforward ways to do so is by additionally train the network over such adversarial examples \cite{SzegedyZSBEGF13CORR}. However,  \cite{SzegedyZSBEGF13CORR}'s algorithm to find such examples for each training sample is computationally expensive and requires long time.  \cite{GoodfellowSS14CORR} proposed a fast alternative to generate adversarial examples using the derivative of the cost function with respect to the input under the form of a regularization as follows
\begin{equation}
    \label{eq:eqapp3-150}
    \widetilde{J}(\bm{\theta}, \xvec, \yvec) = \alpha J(\bm{\theta}, \xvec, \yvec) + (1 - \alpha) J(\bm{\theta}, \xvec + \epsilon \sign(\nabla_{\xvec} J(\bm{\theta}, \xvec, \yvec))) \; ,
\end{equation}
\noindent where $\alpha$ is a regularization decay. Using Eq.\ref{eq:eqapp3-150} to train a neural network allows to reduce the generalization error and reduces its sensibility to adversarial examples \cite{GoodfellowSS14CORR}.

\section{Tangent Propagation}
\label{sec:tangentdistanceapp3}
Manifold assumption \cite{Chapelle2010semisupervisedl} assumes that data in high dimensional space lies in a low dimensional manifold. Therefore, one can take advantage of this hypothesis by working in a low dimensional manifold instead of the whole data space. One way to do so is by using tangent distance \cite{simard1993, Simard1998} which is a nonparameteric nearest neighbor algorithm. Instead of using a generic metric such as the Euclidean distance, tangent distance derives a measure from a prior knowledge of the manifold where the data concentrates. In the context of a classification task, the idea is to find the closest prototype $\xvec^p$ to a test samples $\xvec^t$. The basic challenge is to make the classifier robust to local variations such as rotation, translation, and scale. Using one sided distance, tangent distance constructs an optimization problem to minimize the distance between the tangent plane of the manifold of $\xvec^p$ and the test point $\xvec^t$. Simply saying, the tangent distance attempts to find the parameters of the different transformation that makes the transformed image of $\xvec^p$ close to $\xvec^t$. In order to compute this distance, one need to enumerate in advance the different possible transformations and their tangent vectors.

Based on the same idea, tangent prop \cite{simVicLeCDen92} use similar idea to train neural networks to make the output $f(\xvec)$ invariant to known factors of variation. These factors  of variation correspond to movements along the manifold near which transformed examples of the same class concentrate. Local invariance toward these movements is achieved through a regularization penalty that constrains the directional derivative of $f$ at $\xvec$ in the directions of the tangent vectors $\bm{v}^{(i)}$ to have relatively small norm \cite{simVicLeCDen92, Goodfellowbook2016}
\begin{equation}
    \label{eq:eqapp3-151}
    \Omega(f) = \sum_i \left((\nabla_{\xvec} f(\xvec)^{\top} \cdot \bm{v}^{(i)}\right)^2 \; .
\end{equation}

\noindent Similar to tangent distance, tangent prop requires the tangent vectors to be defined a prior based on the formal knowledge of the effect of the transformations on the input signal. Tangent prop has been used for supervised learning \cite{simVicLeCDen92} as well as in the context of reinforcement learning \cite{Thrun1995}.

Tangent propagation is slightly related to data augmentation. In both methods, one needs to encode some prior knowledge about the task by specifying a set of transformations that should not alter the output of the network. However, in the case of data augmentation, the network is explicitly trained to correctly classify distinct inputs that are created using a set of transformations, usually non-infinitesimal. While tangent propagation does not require explicitly visiting a new input point. Instead, the network is analytically regularized to be invariant to perturbations in some specific directions. Despite its insightful conception, tangent propagation still has some limitations. First, it only regularizes the model to resist infinitesimal perturbations whereas data augmentation encourages resistance to large variations. Second, the infinitesimal approach poses difficulties for models based on rectifier linear units which are enable to keep their gradient invariant in the opposite to sigmoid or hyperbolic tangent units. Whereas, data augmentation tends to work well with rectifier linear unit \cite{krizhevsky12}.

The manifold tangent classifier \cite{RifaNIPS2011} eliminates the need to known the tangent vectors a prior. Instead, the authors use auto-encoders to estimate them in an unsupervised way. This makes this approach easy to use. However, the need to use auto-encoders beforehand may increases the computation cost.

By this, we close this appendix. More on the regularization of neural networks can be found in \cite{Goodfellowbook2016}.
